# Supplementary material for: Generators and Relations for Real Stabilizer Operators
Source: arXiv:2109.05655 ancillary file (2021-09-13)

# Supplement: Generators and Relations for Real Stabilizer Operators

Justin Makary, Neil J Ross, and Peter Selinger

Department of Mathematics and Statistics  
Dalhousie University, Halifax, Canada

This supplement to “Generators and Relations for Real Stabilizer Operators” establishes that the reduced relations of Definition 5.6 imply the typed relations of Definition 5.1 (as listed in the 8 figures, from Figure 3 to Figure 10 in Appendix B).

## 1 Proof of Proposition 5.7

We show that the typed relations, viewed as relations between un-typed circuits, follow from the reduced relations. That is, in this appendix, we *forget* the typing.

Once typing is forgotten, the relations in Figure 6 and Figure 7 coincide so that it is sufficient to derive those in Figure 6. Similarly, of the first 8 rules in Figure 4, the left column is identical to the right column as un-typed rules, so we only prove the left column. Lastly, the next 12 rules of Figure 6 are identical to the 12 rules following them as un-typed rules, so we only derive the first 12 of them.

We start by proving a few useful lemmas before deriving the typed relations. For each one of Figures 3–10, we number the relations left-to-right and row-by-row in order to conveniently refer to them.

### 1.1 Lemmas

**Lemma 1.1.** *The following is a consequence of R2 and R3.*

$$\boxed{H} \bullet \boxed{H} \boxed{H} \bullet \boxed{H} = \text{———} \quad (\text{L1})$$

**Lemma 1.2.** *The following rules are a consequence of R1 – R18*

$$\begin{array}{c} \boxed{H} \text{---} \bullet \text{---} \boxed{H} \boxed{H} \text{---} \bullet \text{---} \boxed{H} \\ \text{---} \bullet \text{---} \text{---} \bullet \text{---} \end{array} = \text{---} \text{---} \quad (\text{L2})$$

$$\begin{array}{c} \text{---} \bullet \text{---} \text{---} \bullet \text{---} \\ \boxed{H} \text{---} \bullet \text{---} \boxed{H} \boxed{H} \text{---} \bullet \text{---} \boxed{H} \end{array} = \text{---} \text{---} \quad (\text{L3})$$

$$\begin{array}{c} \text{---} \bullet \text{---} \bullet \text{---} \boxed{H} \text{---} \bullet \text{---} \\ \boxed{H} \text{---} \bullet \text{---} \boxed{H} \text{---} \bullet \text{---} \boxed{H} \end{array} = \begin{array}{c} \bullet \text{---} \boxed{H} \text{---} \bullet \text{---} \boxed{H} \text{---} \bullet \text{---} \boxed{H} \boxed{H} \text{---} \bullet \text{---} \boxed{H} \\ \bullet \text{---} \boxed{H} \text{---} \bullet \text{---} \text{---} \end{array} \quad (\text{L4})$$

$$\begin{array}{c} \boxed{H} \text{---} \bullet \text{---} \boxed{H} \text{---} \bullet \text{---} \boxed{H} \text{---} \bullet \text{---} \\ \text{---} \bullet \text{---} \text{---} \bullet \text{---} \boxed{H} \end{array} = \begin{array}{c} \bullet \text{---} \boxed{H} \text{---} \bullet \text{---} \text{---} \\ \bullet \text{---} \boxed{H} \text{---} \bullet \text{---} \boxed{H} \text{---} \bullet \text{---} \boxed{H} \boxed{H} \text{---} \bullet \text{---} \boxed{H} \end{array} \quad (\text{L5})$$

$$\begin{array}{c} \bullet \text{---} \boxed{H} \text{---} \bullet \text{---} \boxed{H} \text{---} \bullet \text{---} \text{---} \\ \bullet \text{---} \boxed{H} \text{---} \bullet \text{---} \boxed{H} \text{---} \bullet \text{---} \boxed{H} \end{array} = \begin{array}{c} \boxed{H} \text{---} \bullet \text{---} \boxed{H} \text{---} \bullet \text{---} \boxed{H} \text{---} \bullet \text{---} \boxed{H} \\ \boxed{H} \text{---} \bullet \text{---} \boxed{H} \text{---} \bullet \text{---} \text{---} \end{array} \quad (\text{L6})$$

$$\begin{array}{c} \boxed{H} \text{---} \bullet \text{---} \boxed{H} \text{---} \bullet \text{---} \text{---} \\ \text{---} \bullet \text{---} \boxed{H} \text{---} \bullet \text{---} \boxed{H} \end{array} = \begin{array}{c} \bullet \text{---} \bullet \text{---} \boxed{H} \text{---} \bullet \text{---} \boxed{H} \text{---} \bullet \text{---} \text{---} \\ \text{---} \bullet \text{---} \bullet \text{---} \boxed{H} \text{---} \bullet \text{---} \boxed{H} \end{array} \quad (\text{L7})$$

$$\begin{array}{c} \bullet \text{---} \text{---} \bullet \text{---} \boxed{H} \text{---} \bullet \text{---} \boxed{H} \text{---} \bullet \text{---} \text{---} \\ \bullet \text{---} \boxed{H} \text{---} \bullet \text{---} \boxed{H} \text{---} \bullet \text{---} \boxed{H} \end{array} = \begin{array}{c} \text{---} \bullet \text{---} \boxed{H} \text{---} \bullet \text{---} \boxed{H} \text{---} \bullet \text{---} \text{---} \\ \boxed{H} \text{---} \bullet \text{---} \boxed{H} \text{---} \bullet \text{---} \boxed{H} \text{---} \bullet \text{---} \text{---} \end{array} \quad (\text{L8})$$

**Lemma 1.3.** *The following rules are a consequence of R1 – R18*

$$\begin{array}{c} \bullet \\ | \\ \boxed{H} \text{---} \bullet \text{---} \boxed{H} \boxed{H} \text{---} \bullet \text{---} \boxed{H} \\ | \\ \bullet \end{array} = \begin{array}{c} \bullet \\ | \\ \boxed{H} \text{---} \bullet \text{---} \boxed{H} \boxed{H} \text{---} \bullet \text{---} \boxed{H} \\ | \\ \bullet \end{array} \quad (\text{L9})$$

[illegible]

[illegible]

$$\begin{array}{c} \text{---} \\ |H| \\ \text{---} \end{array} \begin{array}{c} \bullet \\ |H| \\ \text{---} \end{array} = \begin{array}{c} \text{---} \\ |H| \\ \text{---} \end{array} \begin{array}{c} \bullet \\ |H| \\ \text{---} \end{array} \quad (\text{L12})$$

$$\begin{array}{c} \bullet \\ | \\ \text{---} \\ | \\ \bullet \\ | \\ \boxed{H} \end{array} = \begin{array}{c} \boxed{H} \bullet \boxed{H} \bullet \\ | \quad | \quad | \\ \text{---} \quad \text{---} \quad \text{---} \\ | \quad | \quad | \\ \bullet \quad \bullet \quad \bullet \\ | \quad | \quad | \\ \boxed{H} \quad \boxed{H} \quad \boxed{H} \end{array} \quad (L13)$$

[illegible]

$$\begin{array}{c} \bullet \\ | \\ \bullet \\ | \\ \bullet \\ | \\ \bullet \end{array} = \begin{array}{c} \bullet \\ | \\ \bullet \\ | \\ \bullet \\ | \\ \bullet \end{array} \quad (L15)$$

$$\begin{array}{c}
\text{---} \\
\text{---} \\
\text{---}
\end{array}
\begin{array}{c}
\bullet \\
\bullet \\
\bullet
\end{array}
\begin{array}{c}
\text{---} \\
\text{---} \\
\text{---}
\end{array}
=
\begin{array}{c}
\text{---} \\
\text{---} \\
\text{---}
\end{array}
\begin{array}{c}
\bullet \\
\bullet \\
\bullet
\end{array}
\begin{array}{c}
\text{---} \\
\text{---} \\
\text{---}
\end{array}
\quad (L16)$$

$$\begin{array}{c}
\text{---} \\
\text{---} \\
\text{---}
\end{array}
\begin{array}{c}
\bullet \\
\bullet \\
\bullet
\end{array}
\begin{array}{c}
\text{---} \\
\text{---} \\
\text{---}
\end{array}
=
\begin{array}{c}
\text{---} \\
\text{---} \\
\text{---}
\end{array}
\begin{array}{c}
\bullet \\
\bullet \\
\bullet
\end{array}
\begin{array}{c}
\text{---} \\
\text{---} \\
\text{---}
\end{array}
\quad (L17)$$

$$\begin{array}{c} \bullet \\ | \\ \bullet - [H] - \bullet \\ | \\ \bullet \end{array} = \begin{array}{c} \bullet \\ | \\ \bullet - [H] - \bullet \\ | \\ \bullet \end{array} \quad \text{(L18)}$$

$$\begin{array}{c} \bullet \\ | \end{array} \text{---} \left[ \begin{array}{ccccc} & H & & H & \\ H & & H & & H \end{array} \right] = \left[ \begin{array}{ccccccc} & & & & & & \\ H & & H & & H & & H \end{array} \right] \quad (\text{L19})$$

## 1.2 Proofs of Lemmas

**L1:**

$$\begin{array}{c}
 \boxed{H} \text{---} \bullet \text{---} \boxed{H} \boxed{H} \text{---} \bullet \text{---} \boxed{H} \text{---} \xrightarrow{R3} \boxed{H} \text{---} \bullet \text{---} \bullet \text{---} \boxed{H} \text{---} \\
 \xrightarrow{R2} \boxed{H} \boxed{H} \text{---} \text{---} \text{---} \\
 \xrightarrow{R3} \text{---} \text{---} \text{---}
 \end{array}$$

**L2:**

$$\begin{array}{c}
 \boxed{H} \text{---} \bullet \text{---} \boxed{H} \boxed{H} \text{---} \bullet \text{---} \boxed{H} \text{---} \xrightarrow{R3} \boxed{H} \text{---} \bullet \text{---} \bullet \text{---} \boxed{H} \text{---} \\
 \text{---} \bullet \text{---} \text{---} \bullet \text{---} \text{---} \text{---} \xrightarrow{R5} \boxed{H} \boxed{H} \text{---} \text{---} \text{---} \\
 \xrightarrow{R3} \text{---} \text{---} \text{---}
 \end{array}$$

**L3:**

$$\begin{array}{c}
 \text{---} \bullet \text{---} \text{---} \bullet \text{---} \text{---} \xrightarrow{R3} \text{---} \bullet \text{---} \bullet \text{---} \text{---} \\
 \boxed{H} \text{---} \bullet \text{---} \boxed{H} \boxed{H} \text{---} \bullet \text{---} \boxed{H} \text{---} \xrightarrow{R5} \boxed{H} \boxed{H} \text{---} \text{---} \text{---} \\
 \xrightarrow{R3} \text{---} \text{---} \text{---}
 \end{array}$$

**L4:**

$$\begin{array}{c}
 \text{---} \bullet \text{---} \text{---} \bullet \text{---} \boxed{H} \text{---} \bullet \text{---} \xrightarrow{R11} \text{---} \bullet \text{---} \bullet \text{---} \bullet \text{---} \boxed{H} \text{---} \bullet \text{---} \\
 \boxed{H} \text{---} \bullet \text{---} \boxed{H} \text{---} \bullet \text{---} \boxed{H} \text{---} \bullet \text{---} \xrightarrow{R3} \text{---} \bullet \text{---} \bullet \text{---} \bullet \text{---} \boxed{H} \text{---} \bullet \text{---} \\
 \xrightarrow{R3} \text{---} \bullet \text{---} \boxed{H} \text{---} \bullet \text{---} \text{---} \text{---} \xrightarrow{R3} \text{---} \bullet \text{---} \bullet \text{---} \boxed{H} \boxed{H} \text{---} \bullet \text{---} \boxed{H} \text{---} \bullet \text{---} \\
 \xrightarrow{R8} \text{---} \bullet \text{---} \bullet \text{---} \boxed{H} \text{---} \bullet \text{---} \boxed{H} \text{---} \bullet \text{---} \boxed{H} \text{---} \bullet \text{---} \xrightarrow{R10} \text{---} \bullet \text{---} \boxed{H} \text{---} \bullet \text{---} \boxed{H} \text{---} \bullet \text{---} \bullet \text{---} \boxed{H} \text{---} \bullet \text{---} \\
 \xrightarrow{R3} \text{---} \bullet \text{---} \boxed{H} \text{---} \bullet \text{---} \boxed{H} \text{---} \bullet \text{---} \boxed{H} \boxed{H} \text{---} \bullet \text{---} \boxed{H} \text{---} \bullet \text{---}
 \end{array}$$

**L5:**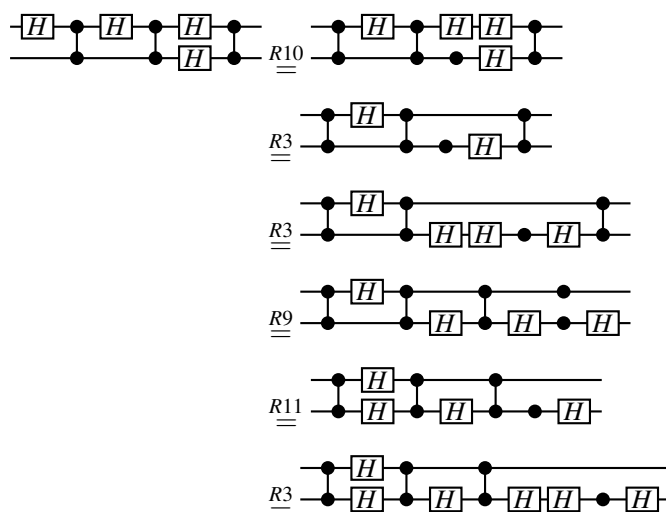**L6:**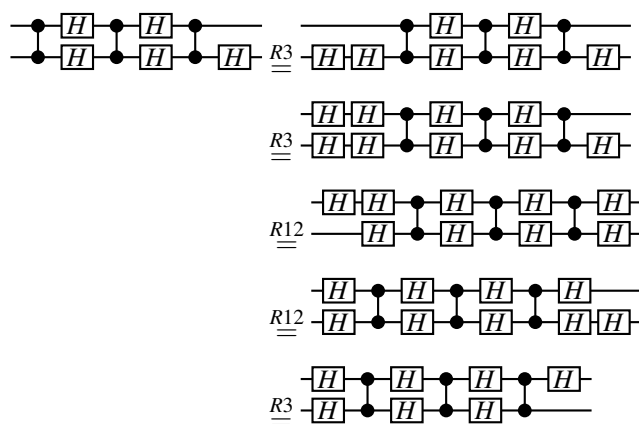

**L7:**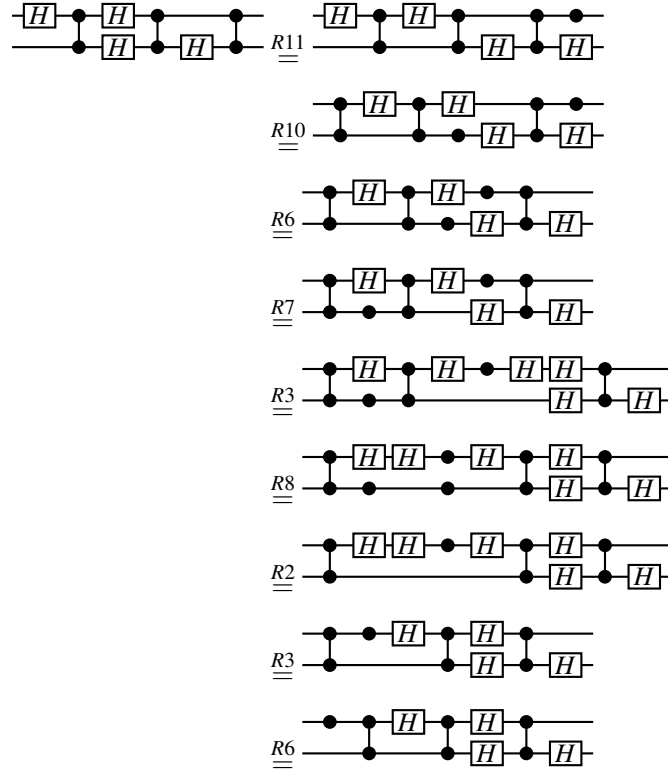

**L8:**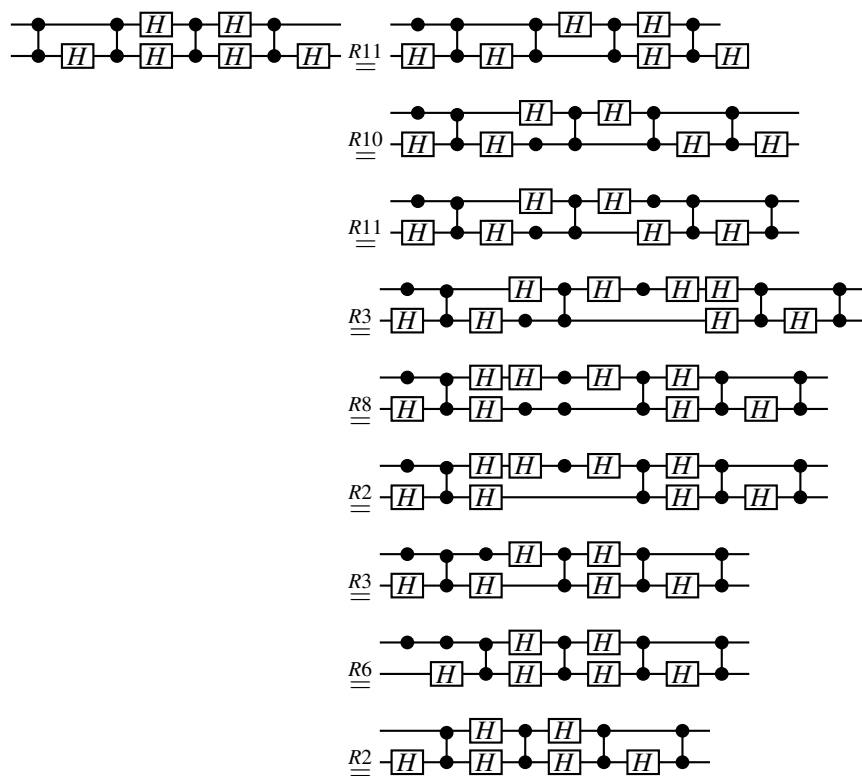**L9:**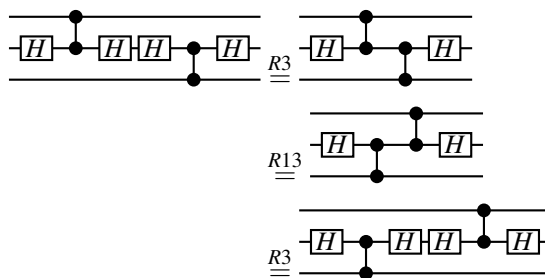

**L10:**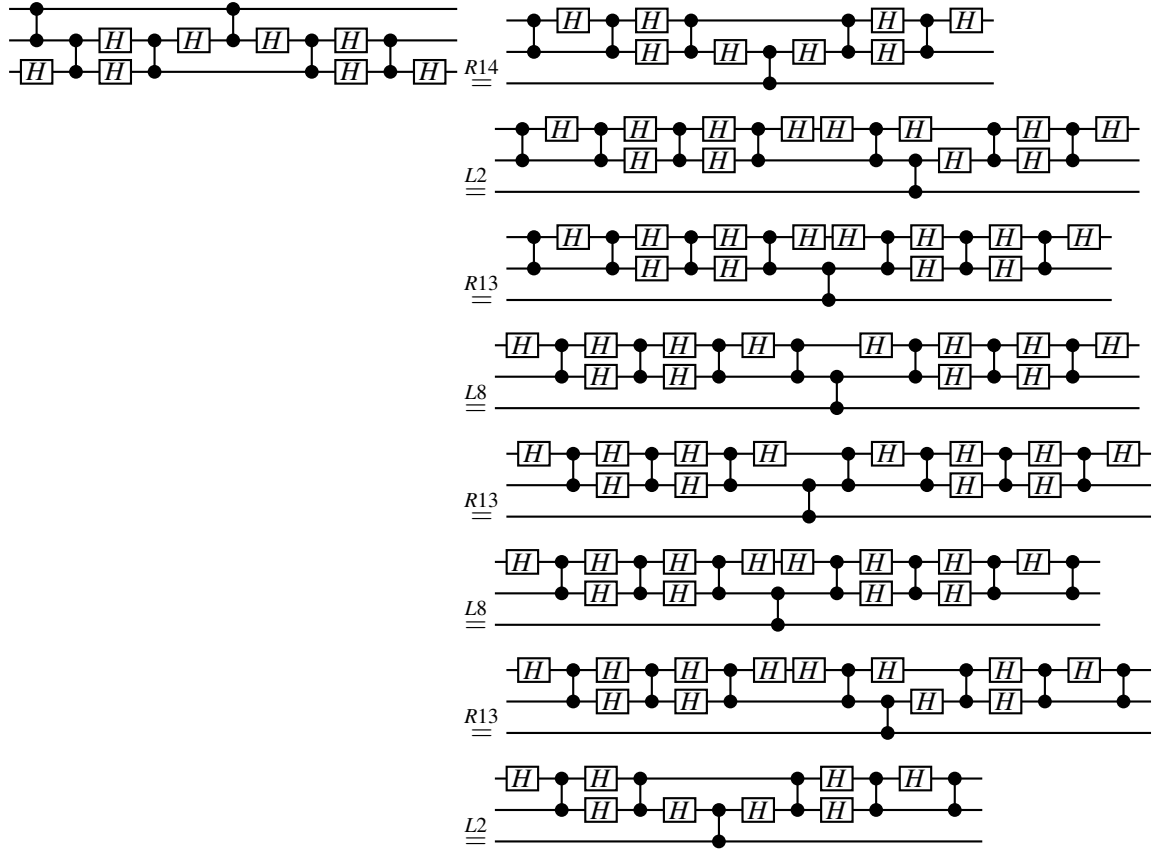

**L11:**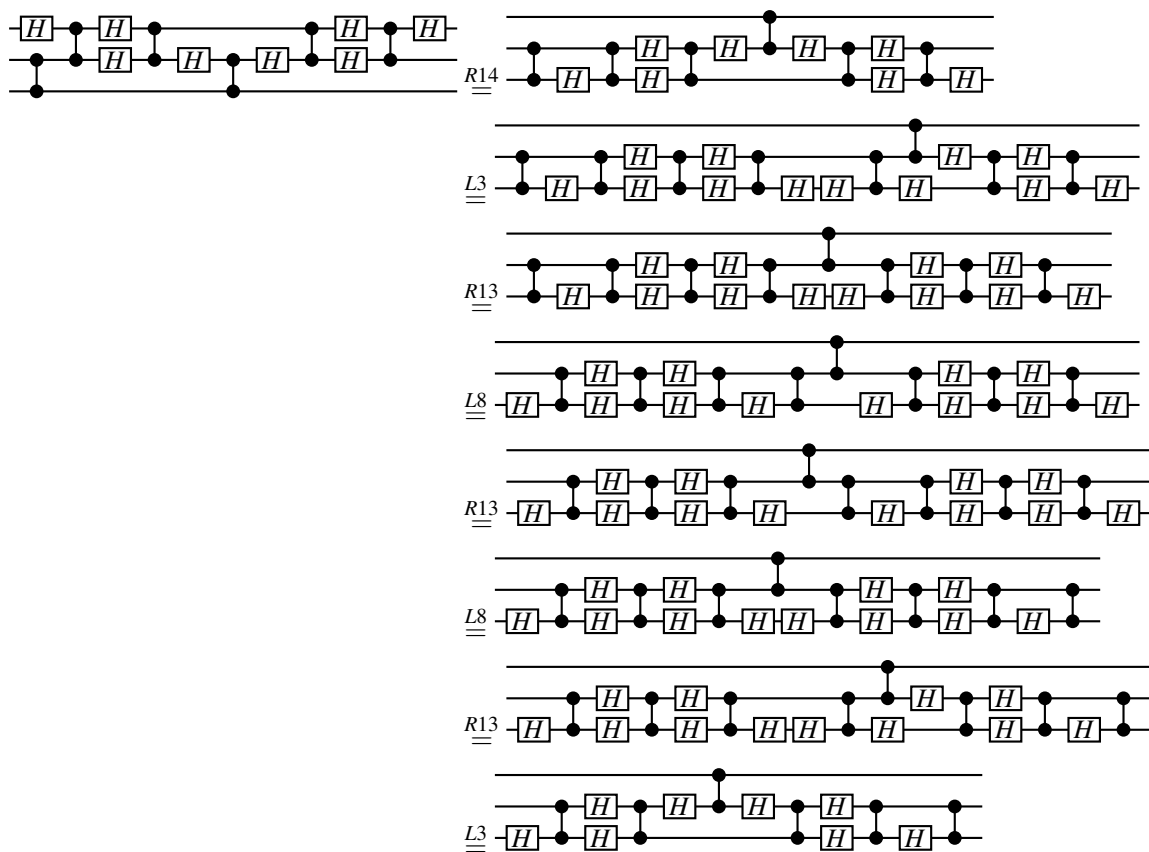

**L12:**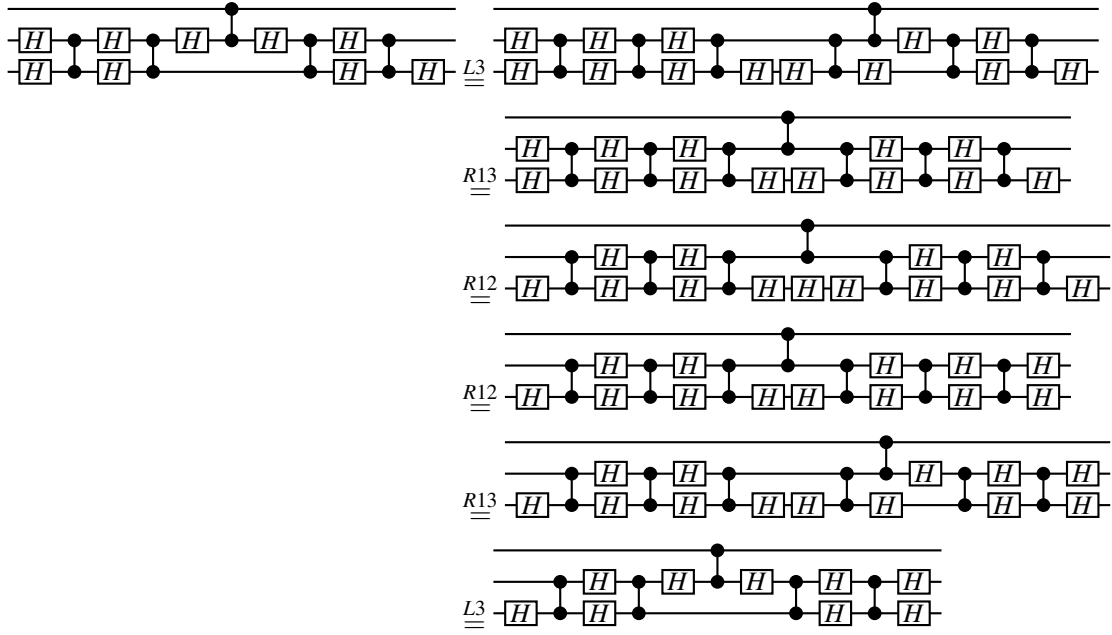

**L13:**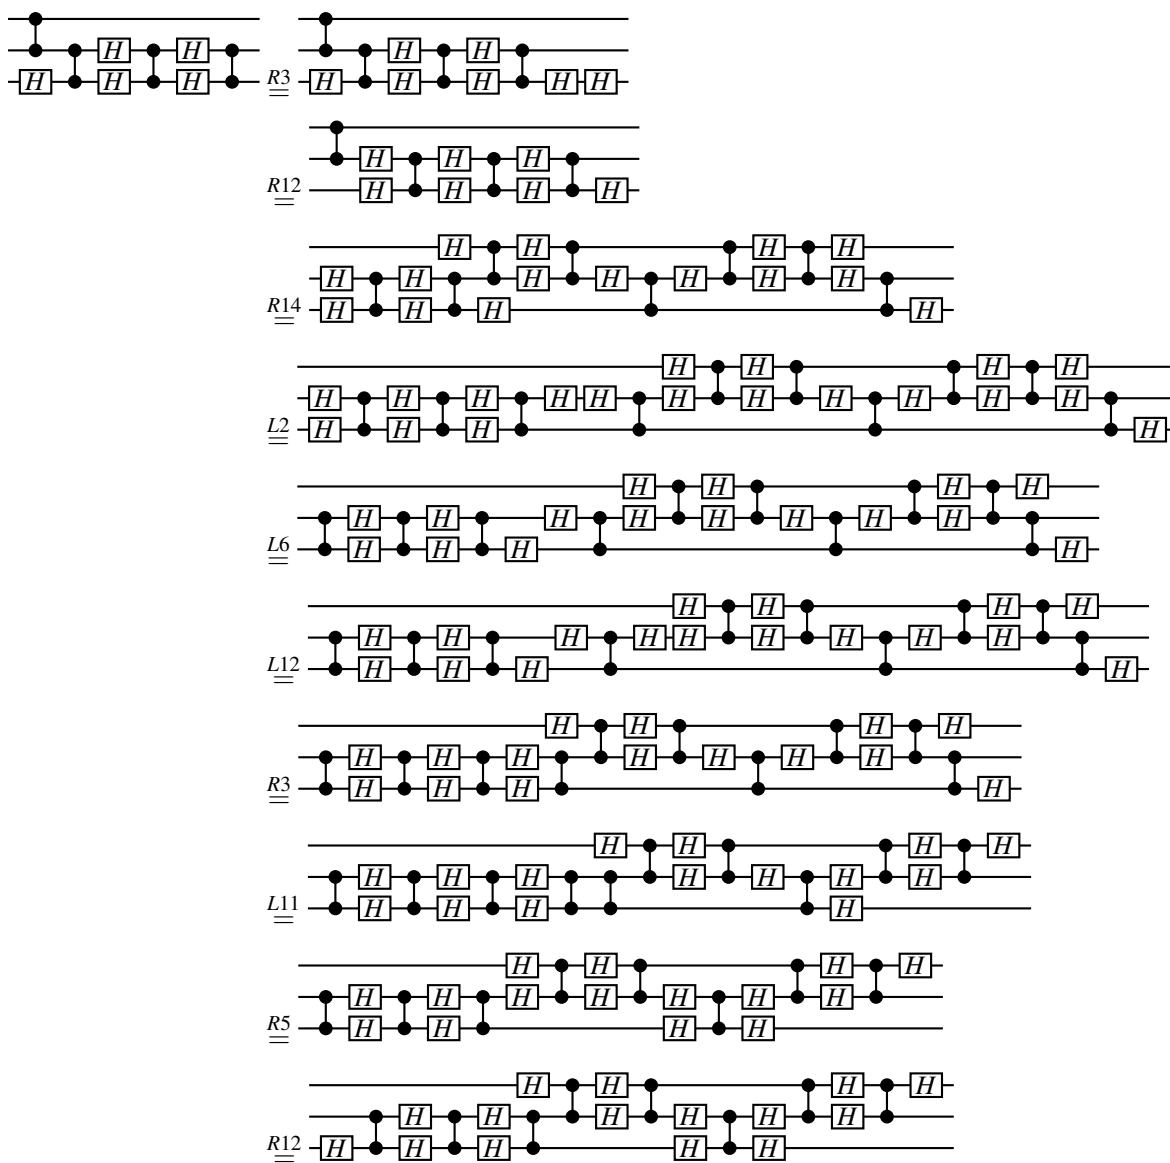

**L14:**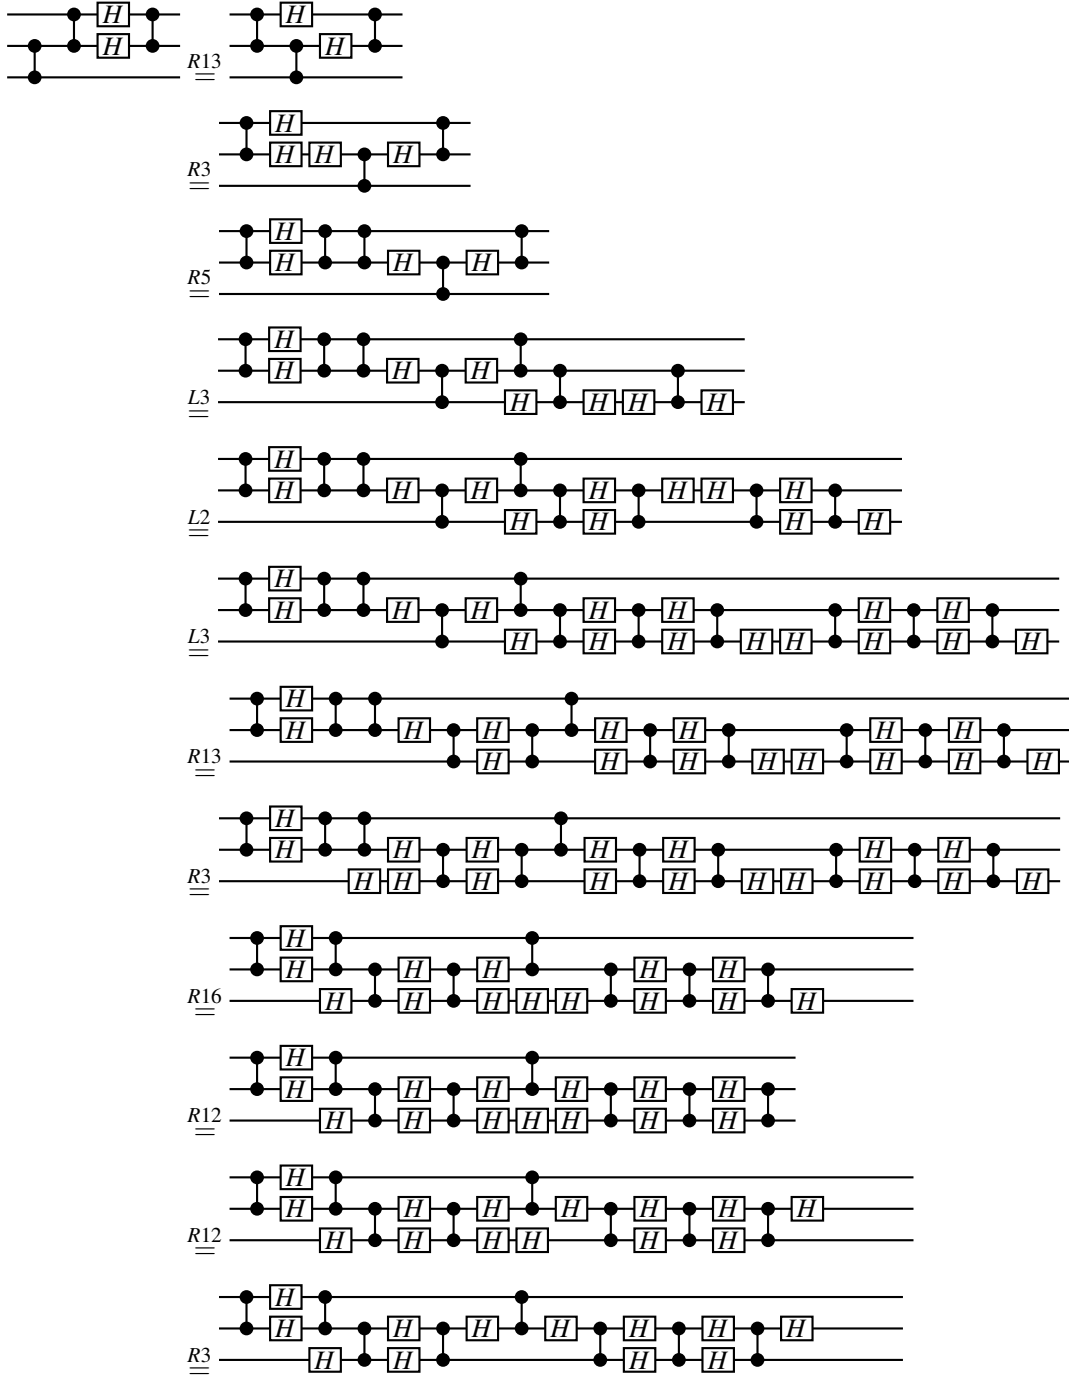

**L15:**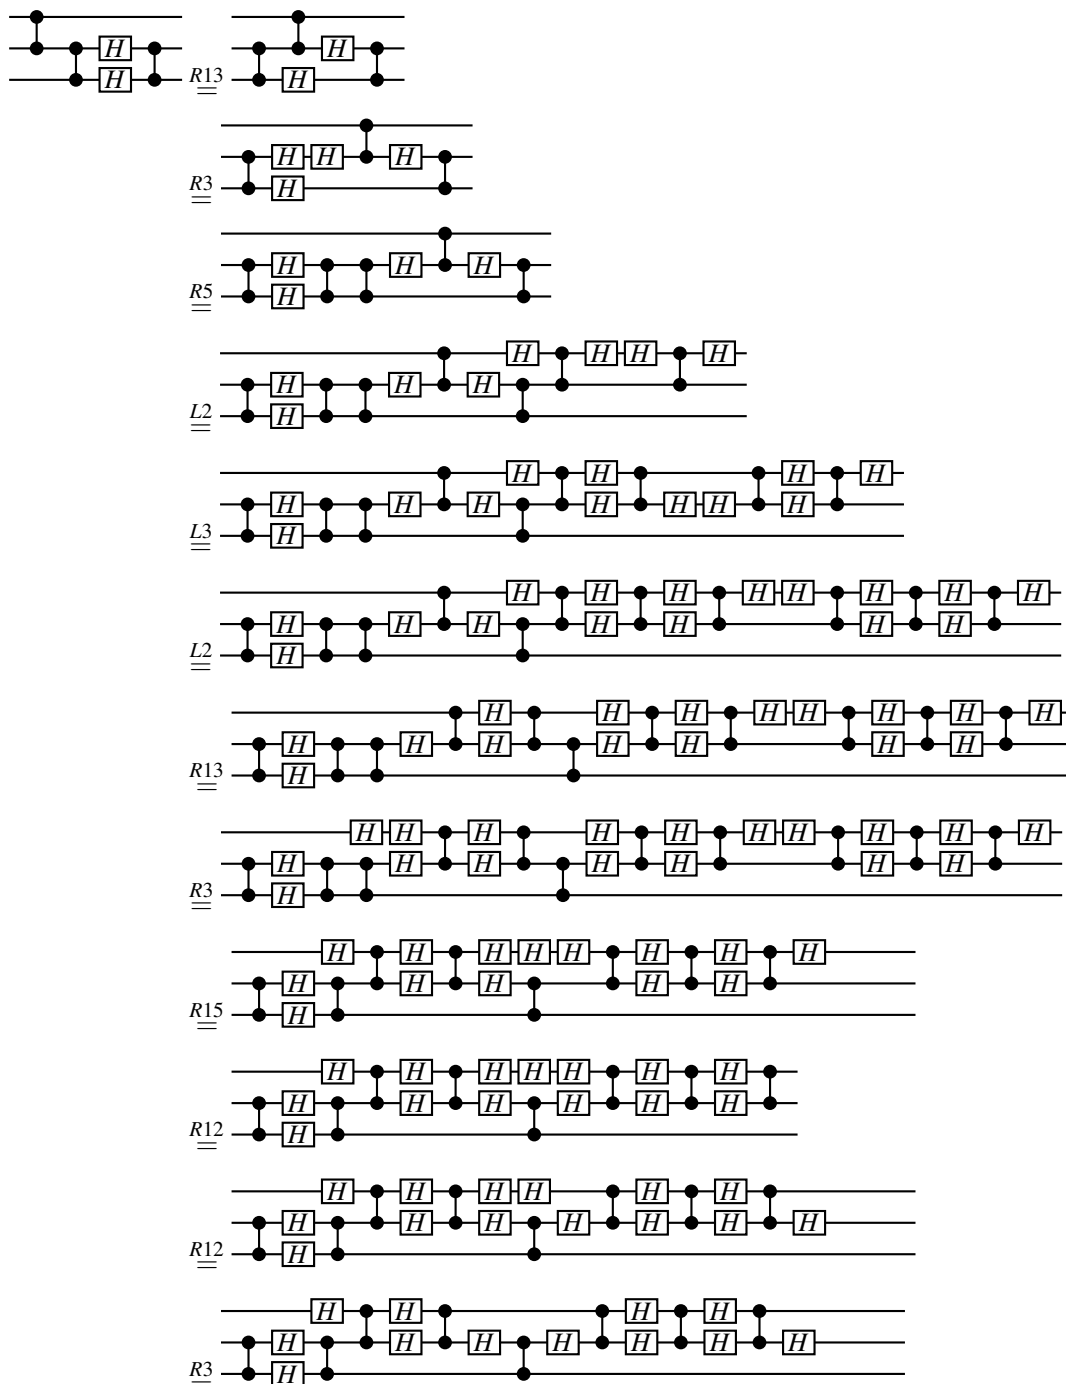

**L16:**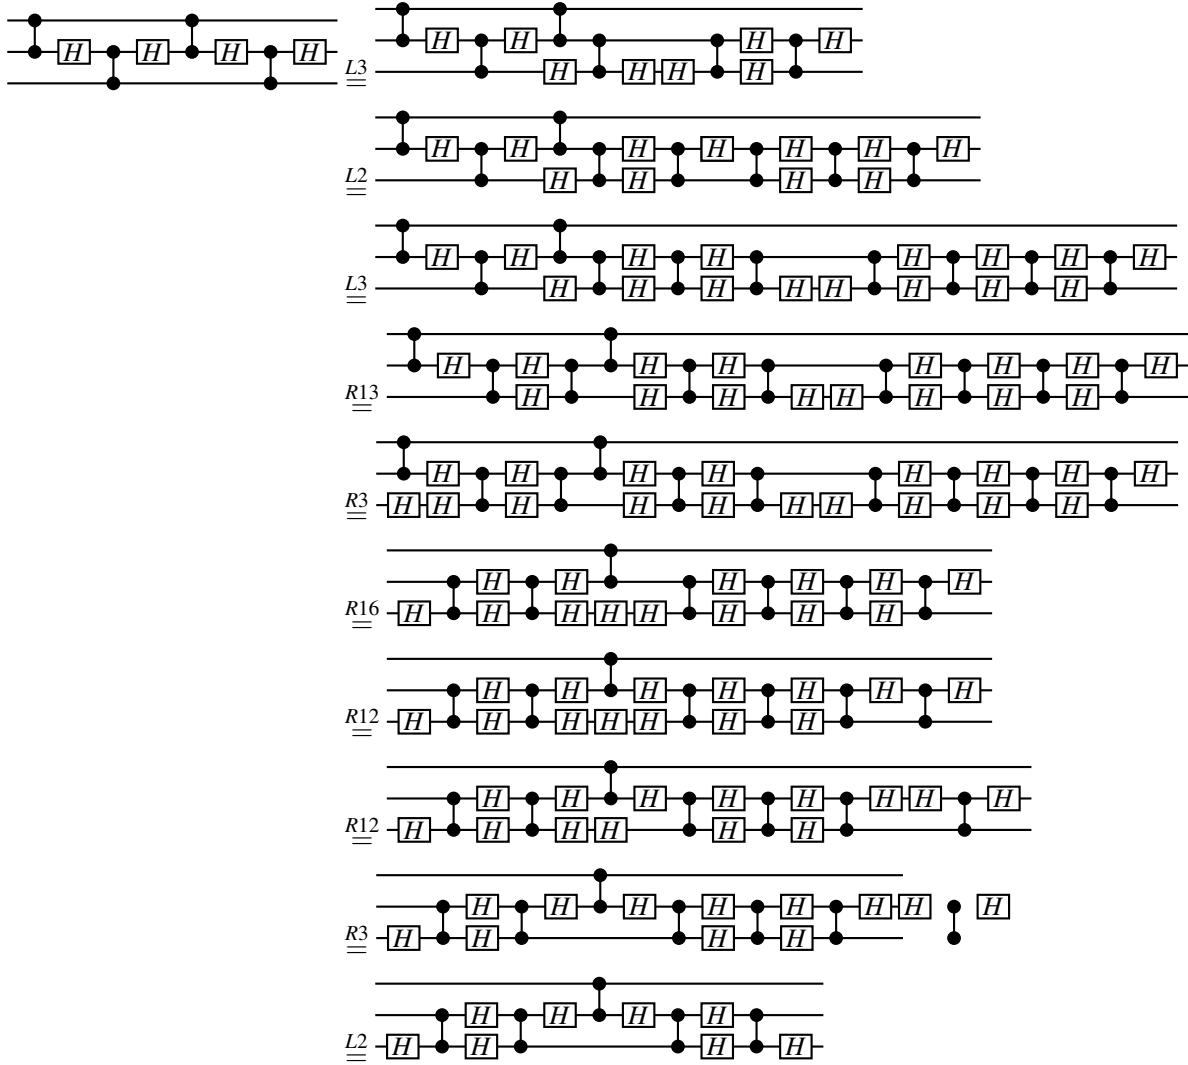

**L17:**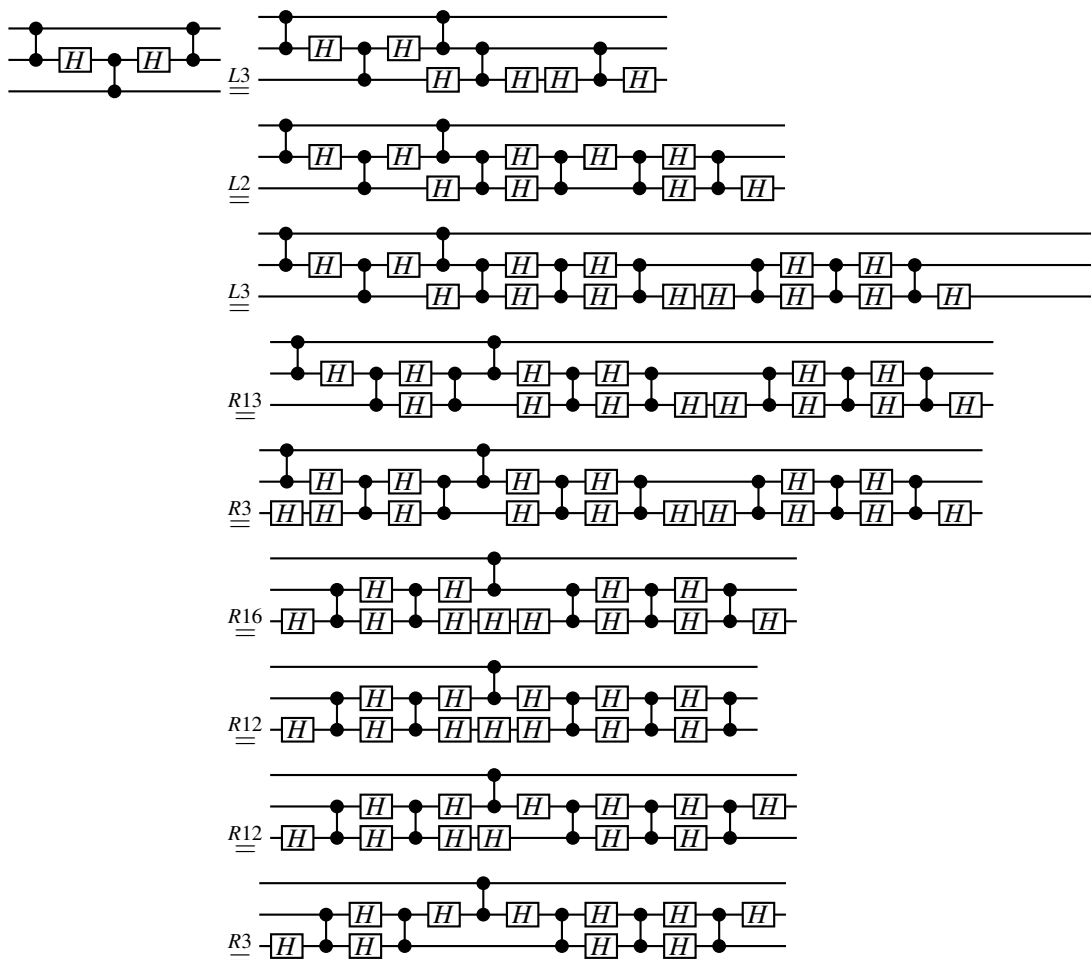

**L18:**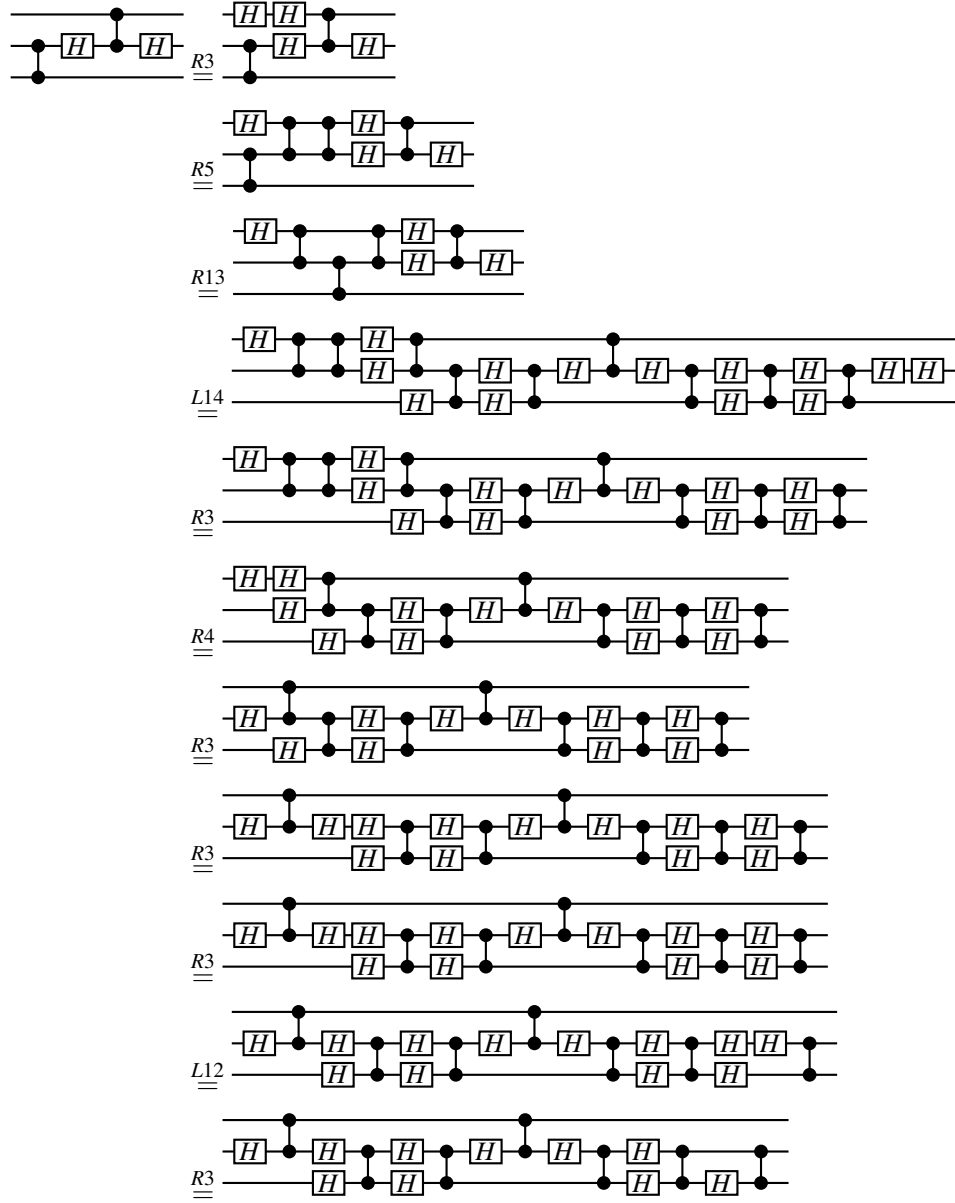

**L19:**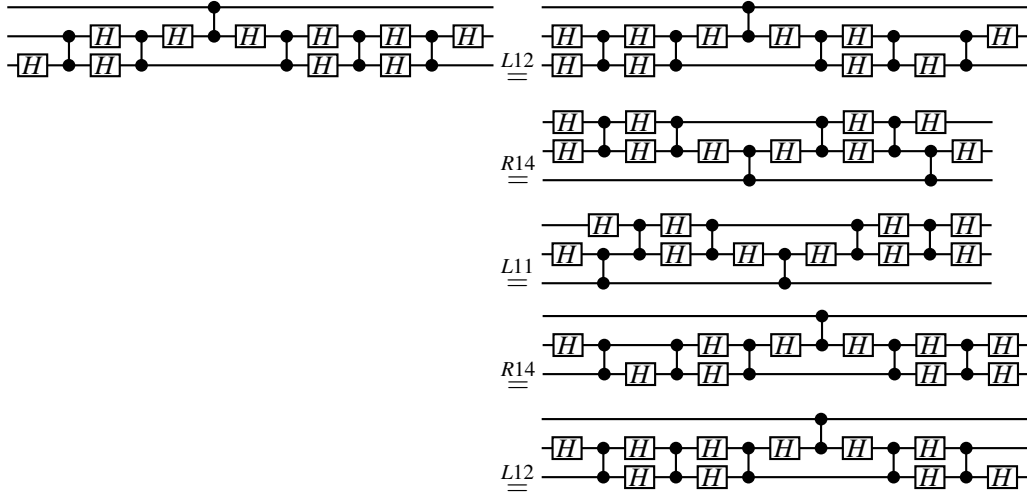

### 1.3 Proofs of Rewrite Rules

**Figure 3:**

3.1

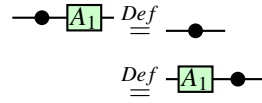

3.2

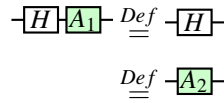

3.3

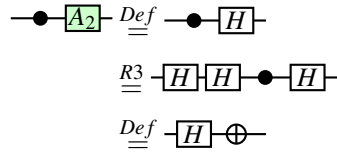

3.4

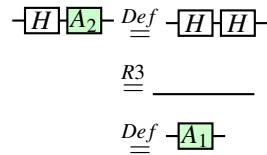

3.5

$$\begin{array}{c}
 \text{---} \bullet \text{---} \boxed{A_3} \text{---} \stackrel{\text{Def}}{=} \text{---} \bullet \text{---} \\
 \stackrel{\text{Def}}{=} \text{---} \stackrel{\text{Def}}{=} \boxed{A_3} \text{---} \bullet \text{---}
 \end{array}$$

3.6

$$\begin{array}{c}
 \text{---} \boxed{H} \boxed{A_3} \text{---} \stackrel{\text{Def}}{=} \text{---} \boxed{H} \text{---} \\
 \stackrel{\text{Def}}{=} \text{---} \stackrel{\text{Def}}{=} \boxed{A_3} \boxed{H} \text{---}
 \end{array}$$

3.7

$$\begin{array}{c}
 \begin{array}{c} \text{---} \bullet \text{---} \boxed{A_1} \text{---} \\ \text{---} \bullet \text{---} \end{array} \stackrel{\text{Def}}{=} \begin{array}{c} \text{---} \bullet \text{---} \\ \text{---} \bullet \text{---} \end{array} \\
 \stackrel{\text{Def}}{=} \begin{array}{c} \text{---} \boxed{A_1} \text{---} \bullet \text{---} \\ \text{---} \bullet \text{---} \end{array}
 \end{array}$$

3.8

$$\begin{array}{c}
 \begin{array}{c} \text{---} \bullet \text{---} \boxed{A_2} \text{---} \\ \text{---} \bullet \text{---} \end{array} \stackrel{\text{Def}}{=} \begin{array}{c} \text{---} \bullet \text{---} \boxed{H} \text{---} \\ \text{---} \bullet \text{---} \end{array} \\
 \stackrel{R3}{=} \begin{array}{c} \text{---} \bullet \text{---} \boxed{H} \text{---} \\ \text{---} \bullet \text{---} \boxed{H} \boxed{H} \text{---} \end{array} \\
 \stackrel{R5}{=} \begin{array}{c} \text{---} \bullet \text{---} \boxed{H} \text{---} \bullet \text{---} \bullet \text{---} \\ \text{---} \bullet \text{---} \boxed{H} \text{---} \bullet \text{---} \bullet \text{---} \boxed{H} \text{---} \end{array} \\
 \stackrel{\text{Def}}{=} \begin{array}{c} \text{---} \boxed{B_2} \text{---} \bullet \text{---} \\ \text{---} \bullet \text{---} \boxed{H} \text{---} \end{array}
 \end{array}$$

3.9

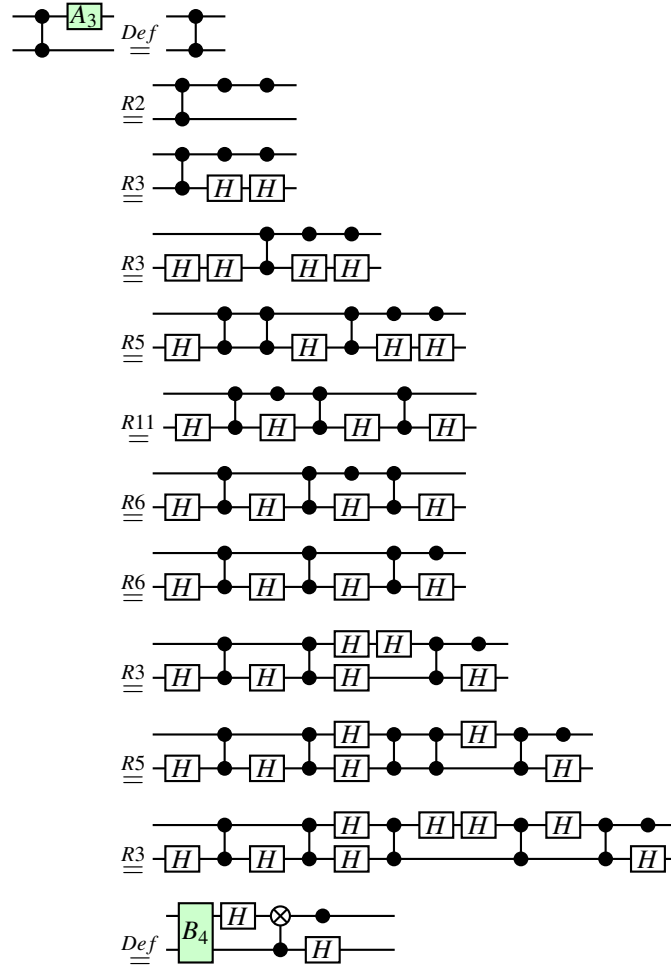

3.10

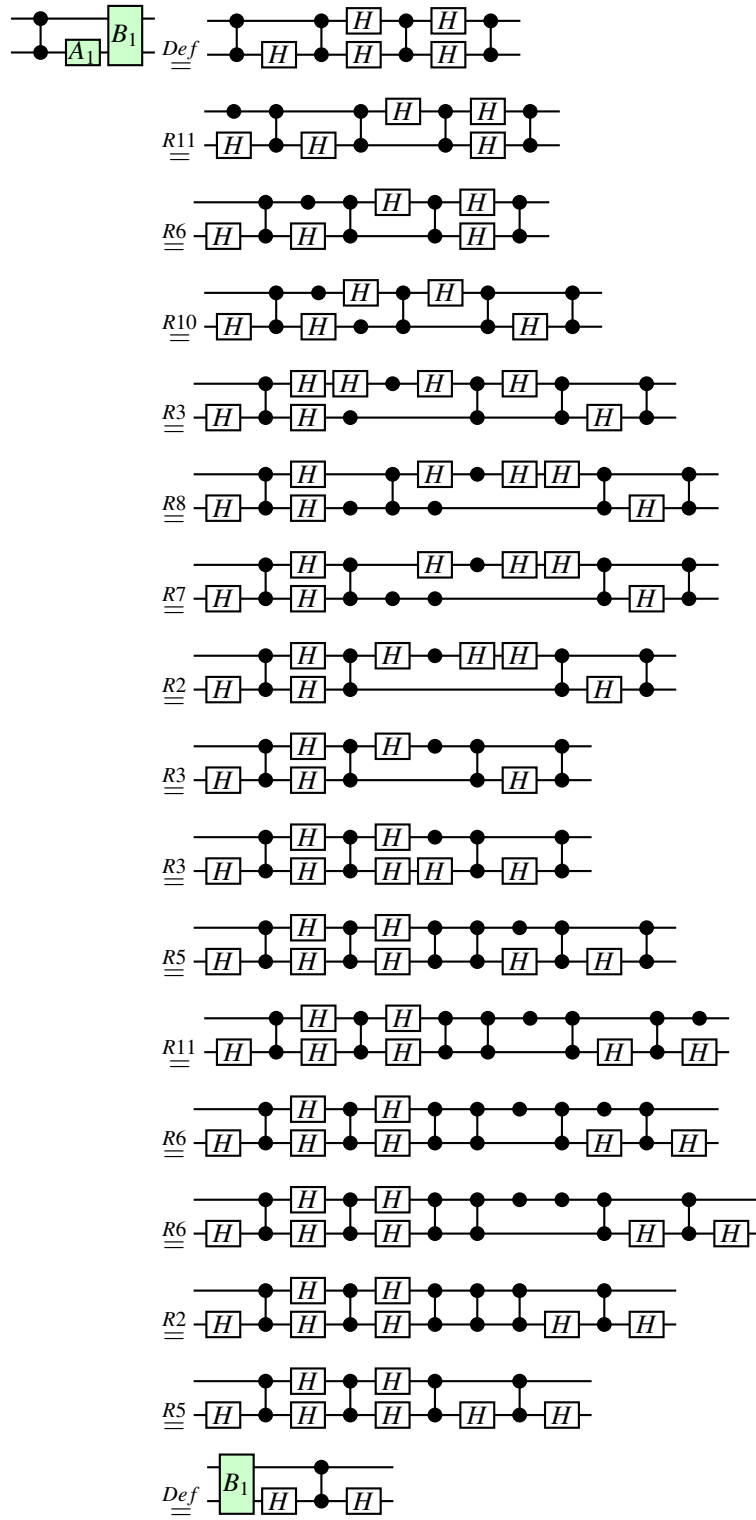

3.11

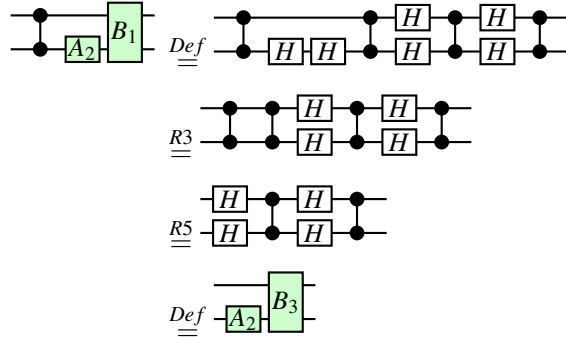

3.12

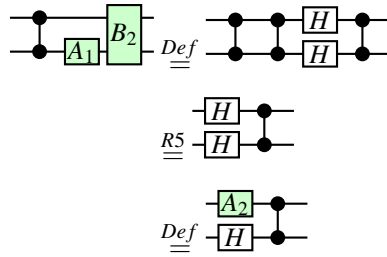

3.13

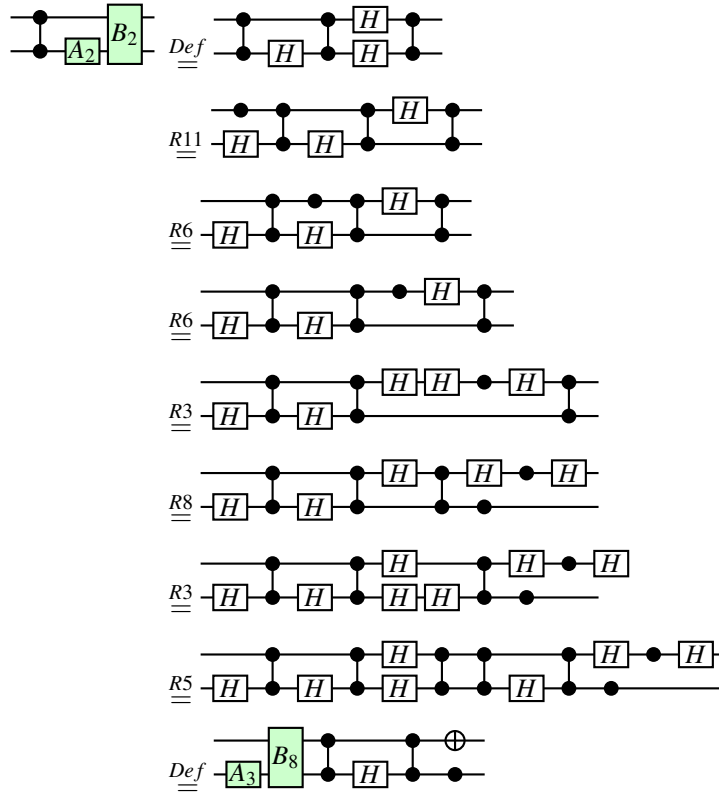

3.14

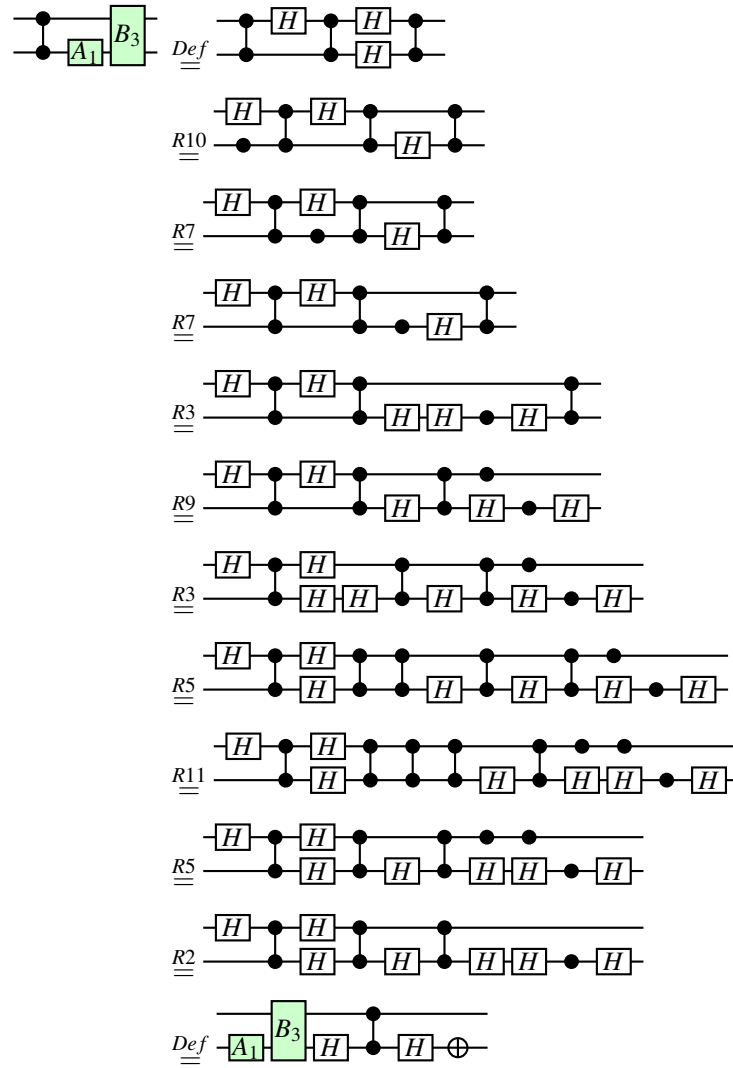

3.15

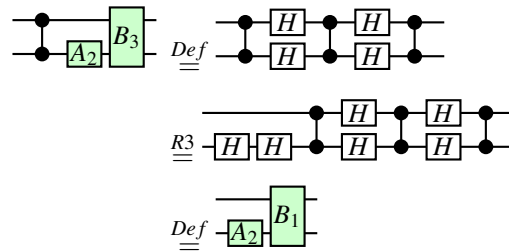

3.16

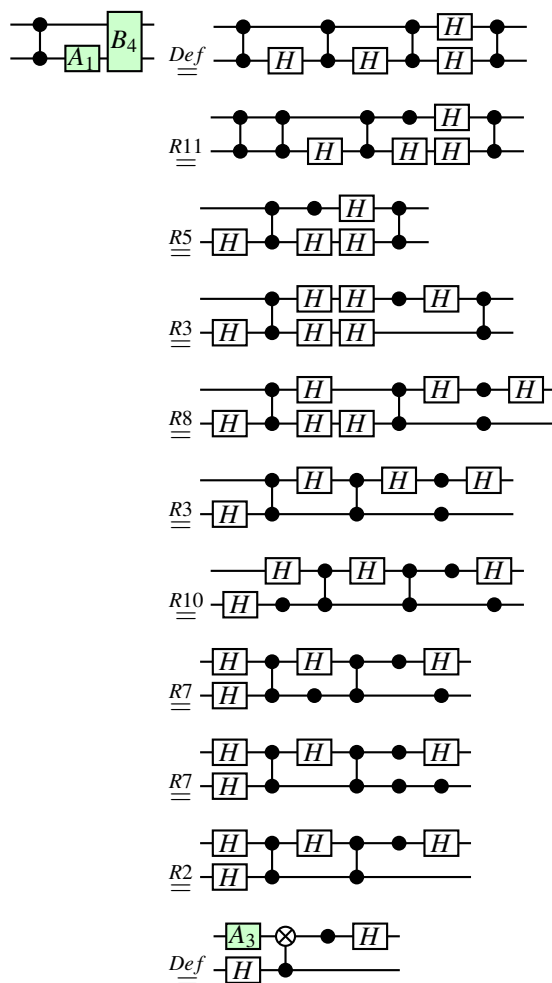

3.17

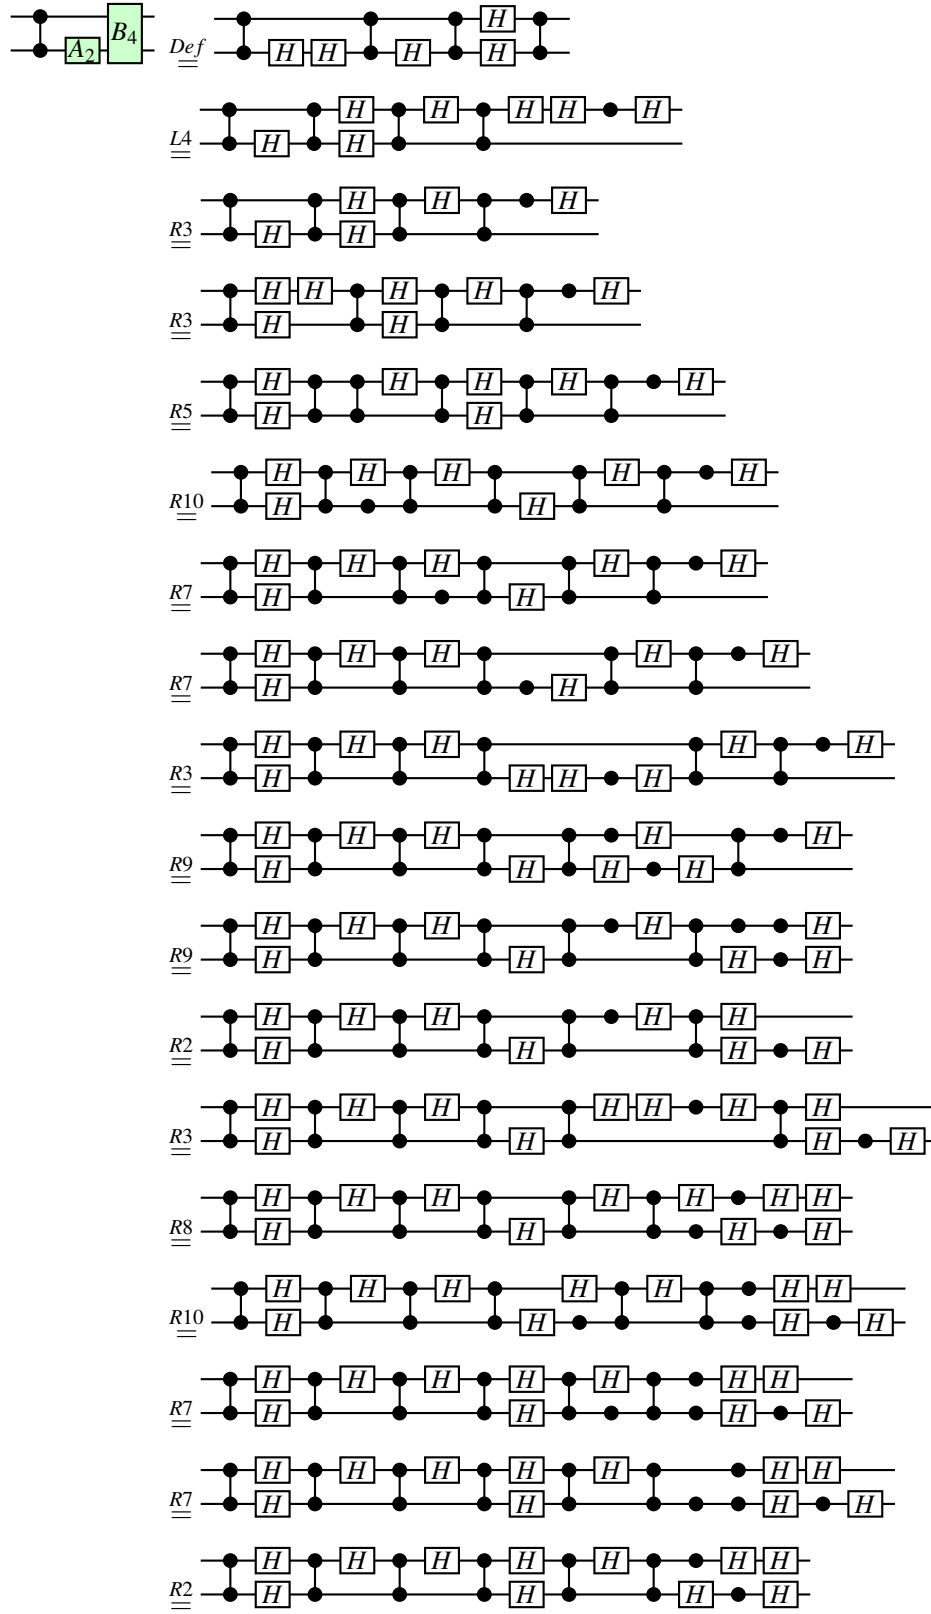

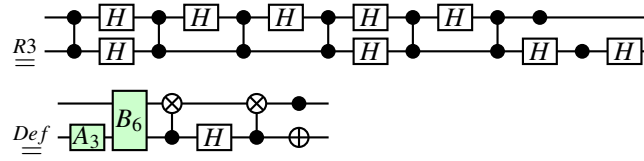

3.18

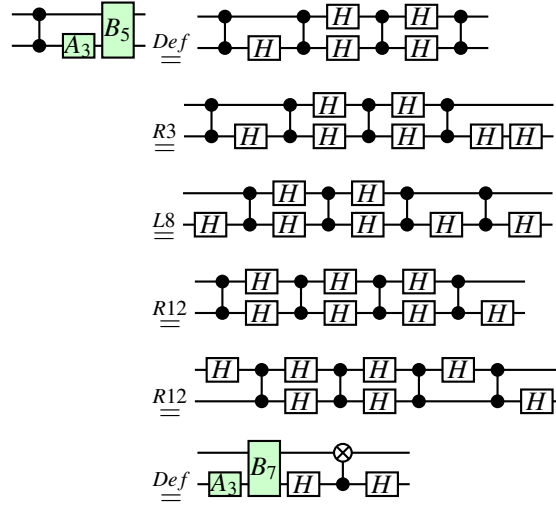

3.19

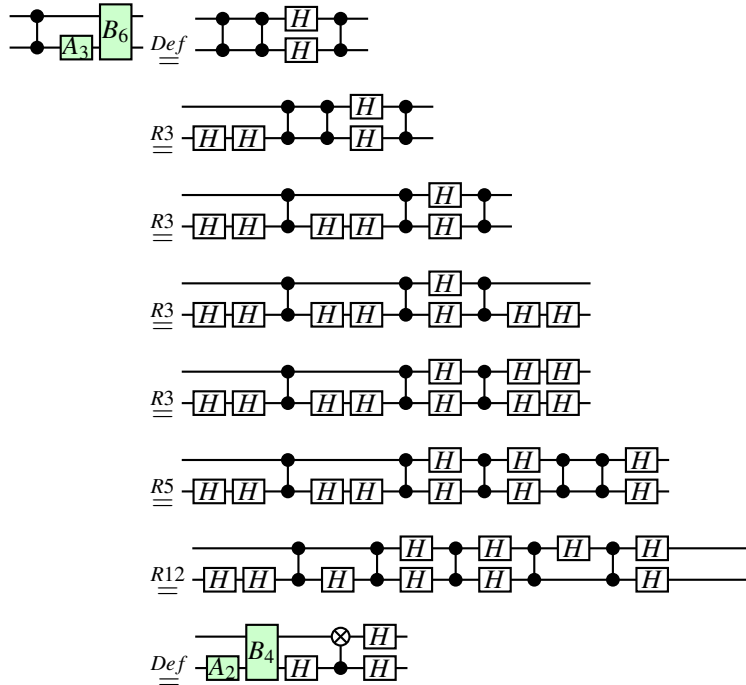

3.20

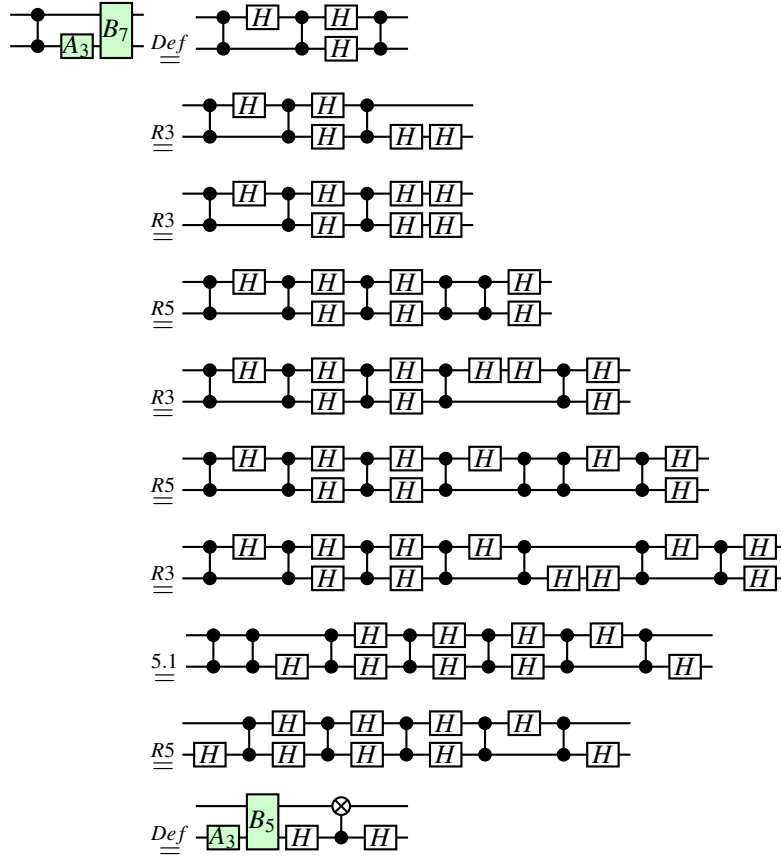

3.21

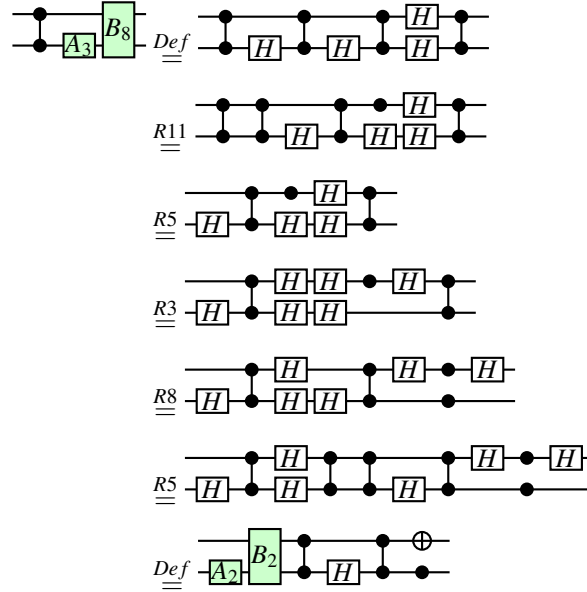

3.22

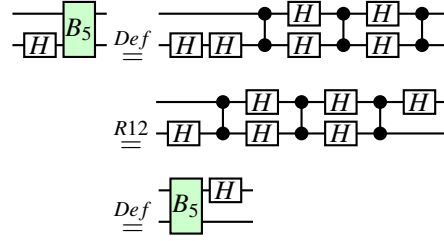

3.23

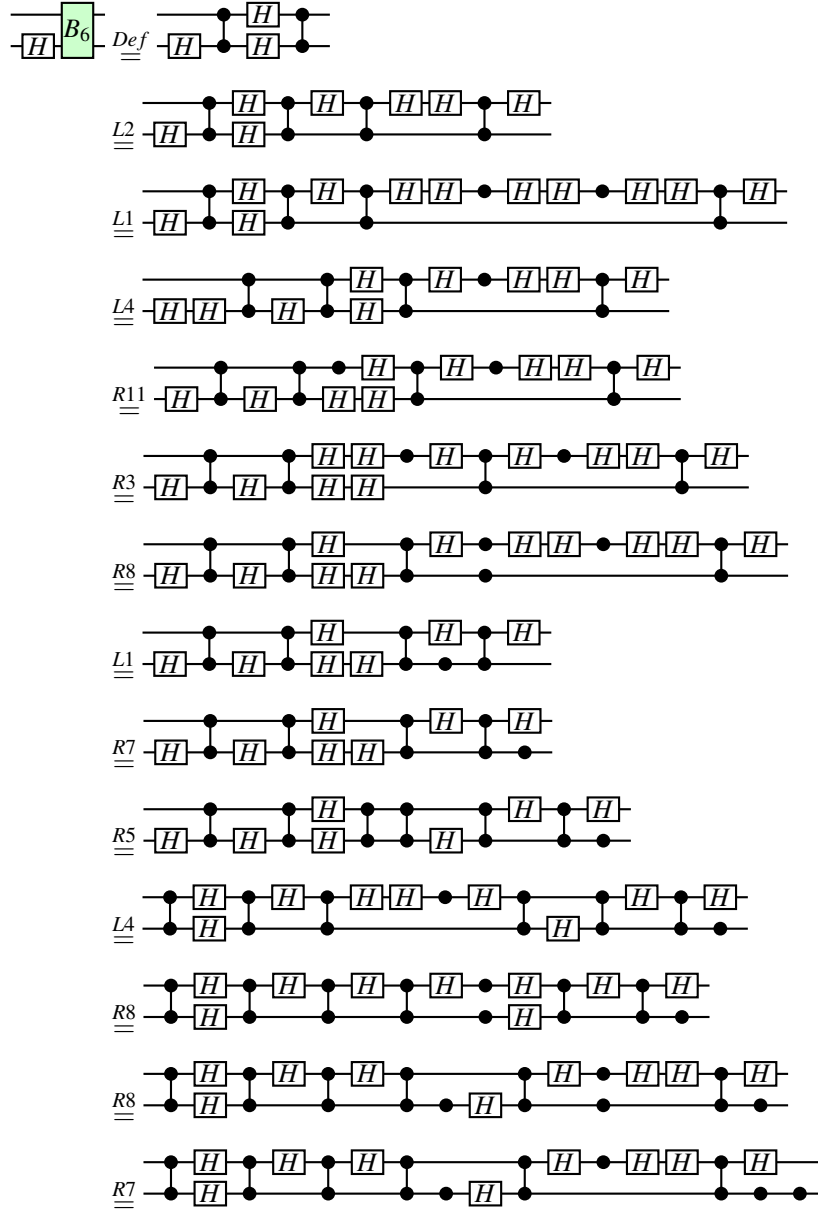

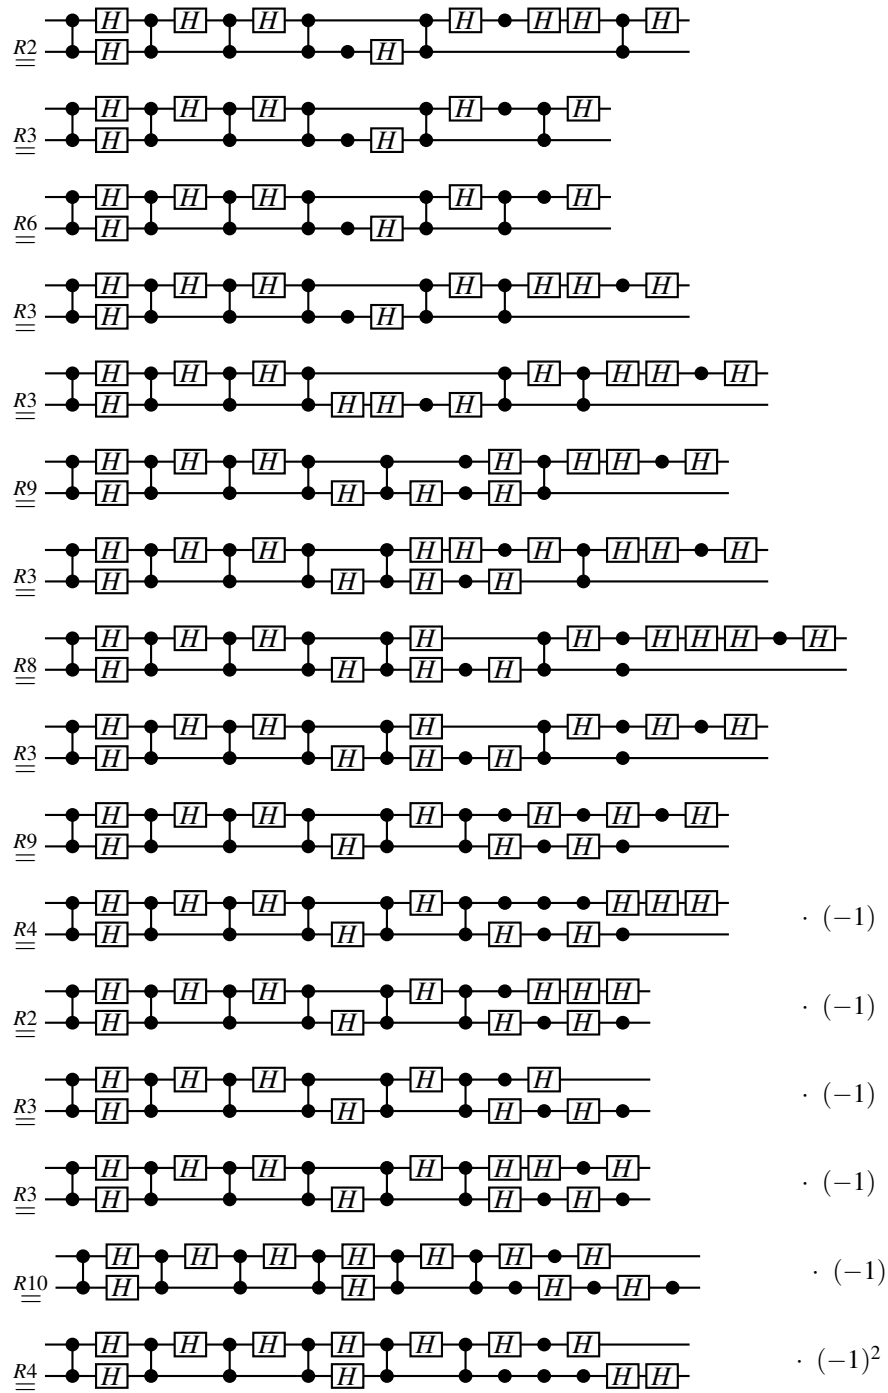

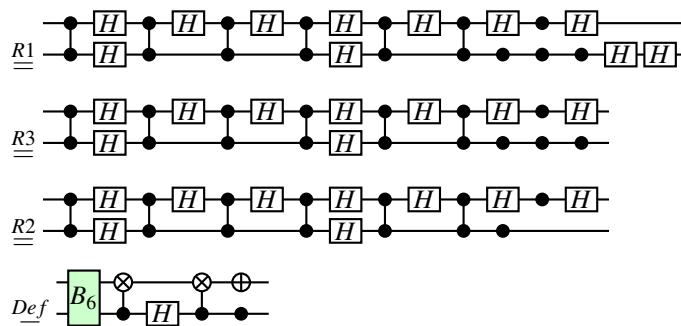

3.24

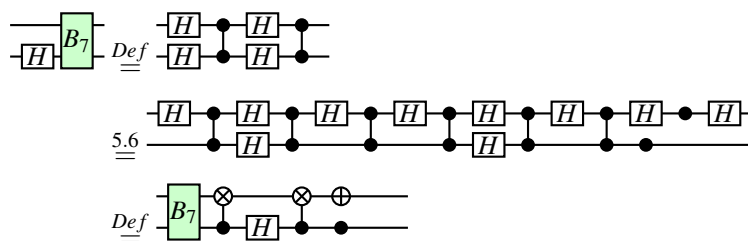

3.25

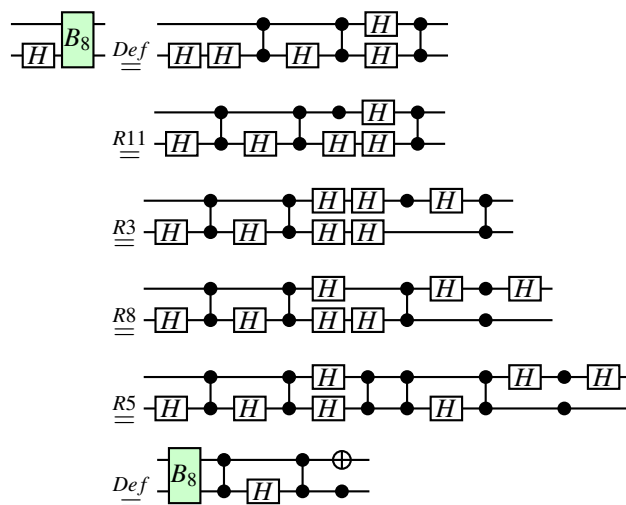

**Figure 4:**

4.1

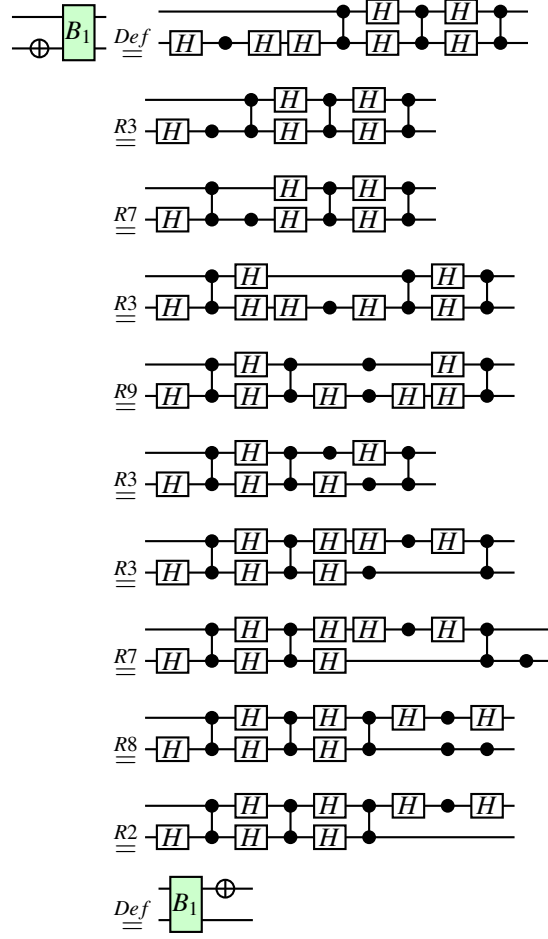

4.2

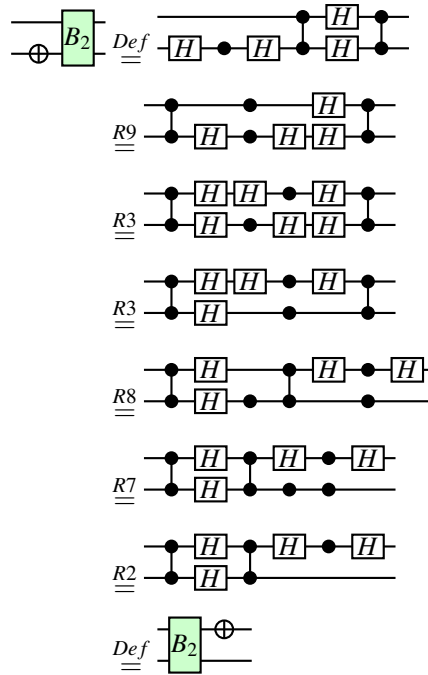

4.3

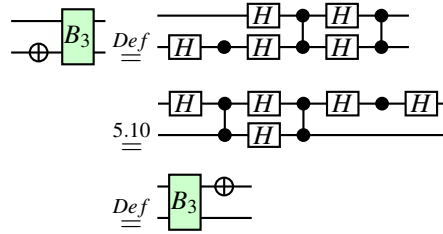

4.4

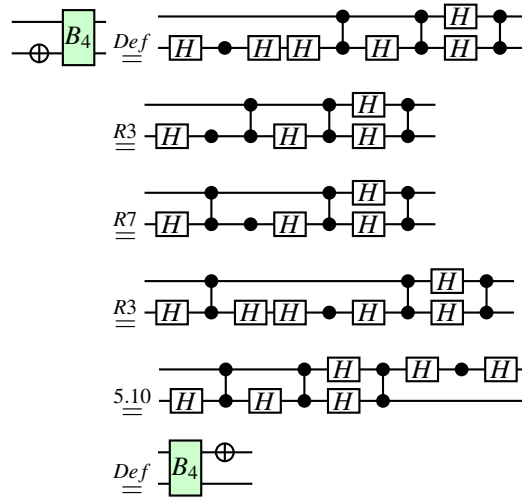

The proofs of 4.5–4.8 are the same as those of 4.1–4.4.

4.9

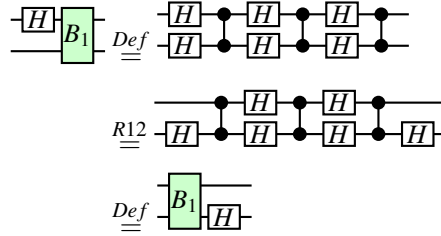

4.10

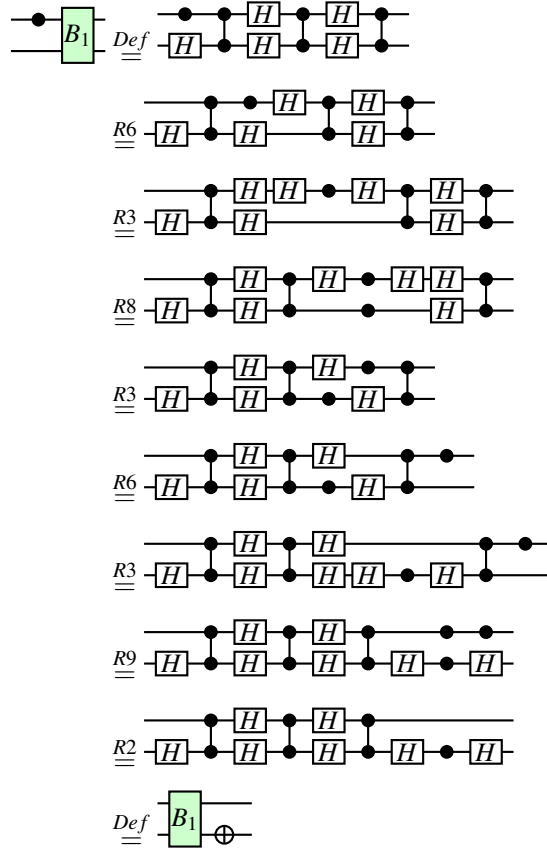

4.11

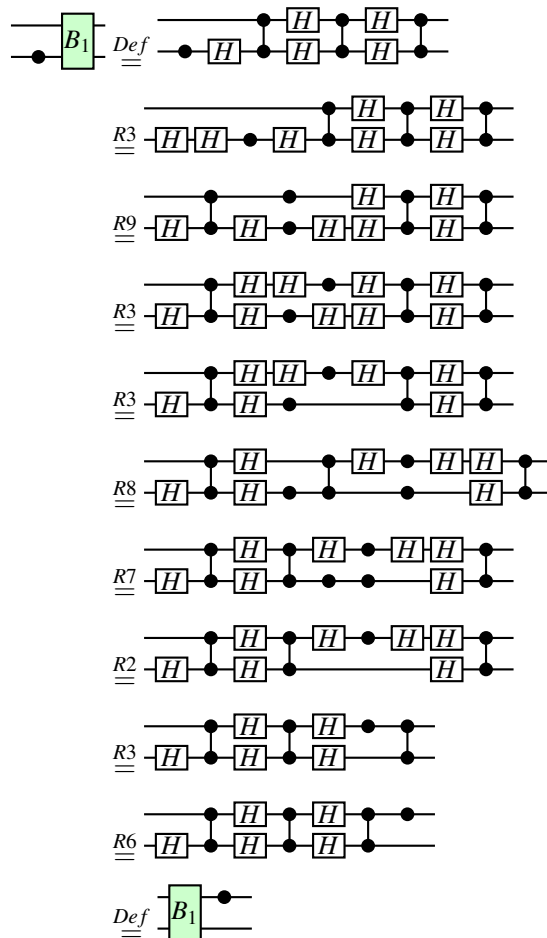

4.12

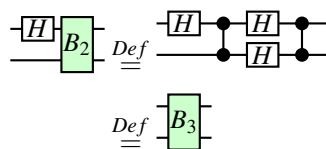

4.13

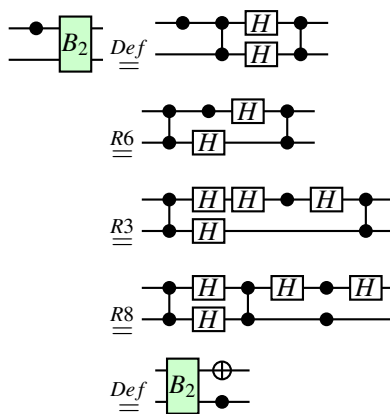

4.14

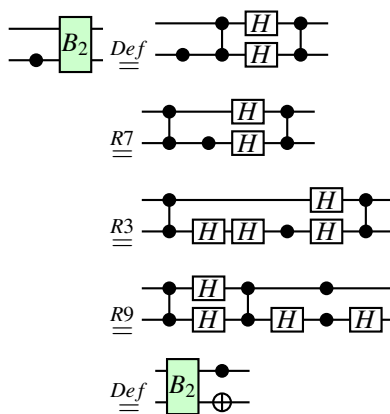

4.15

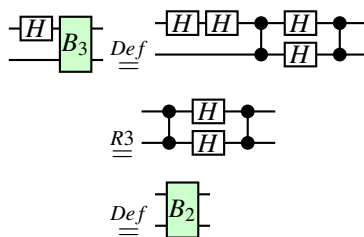

4.16

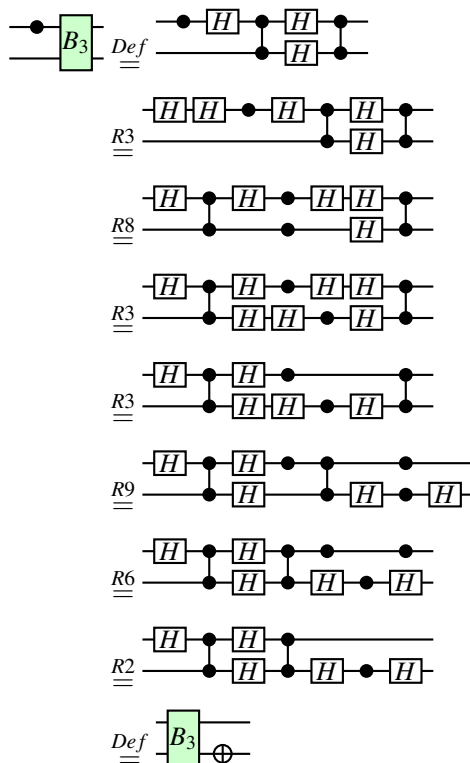

4.17

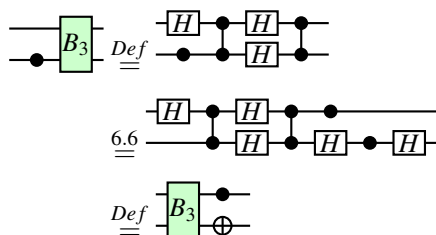

4.18

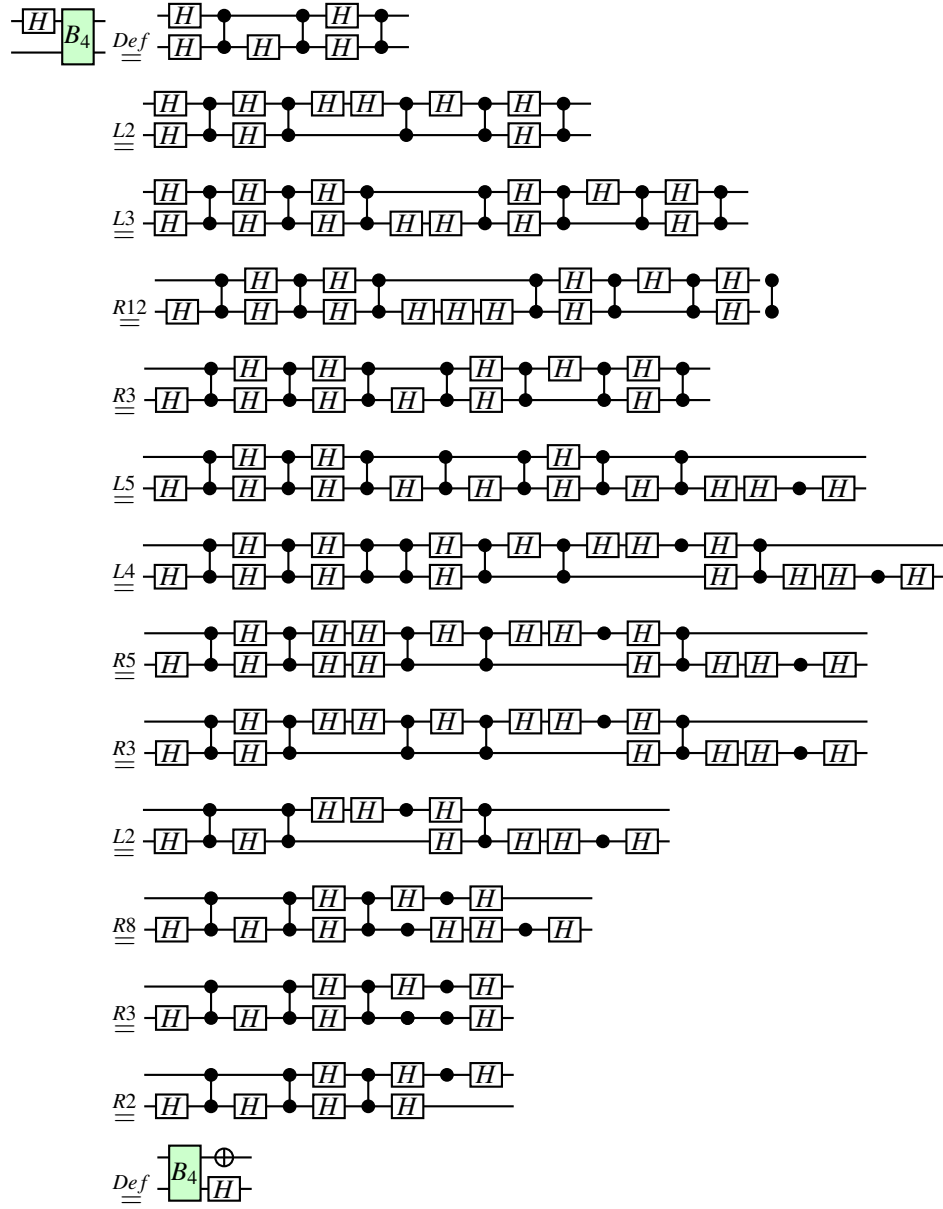

4.19

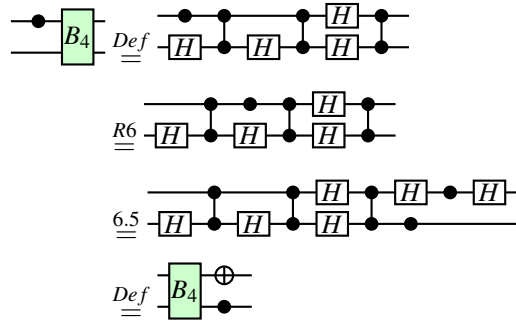

4.20

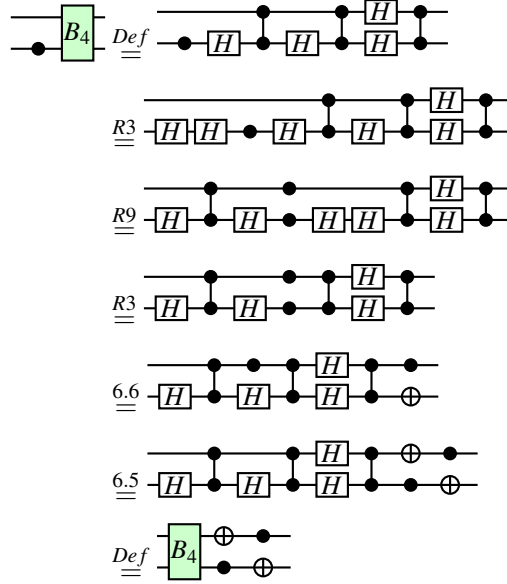

The proofs of 4.21–4.32 are the same as those of 4.9–4.20.

4.33

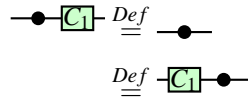

4.34

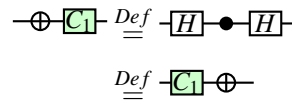

4.35

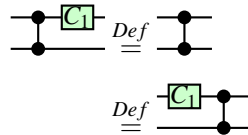

4.36

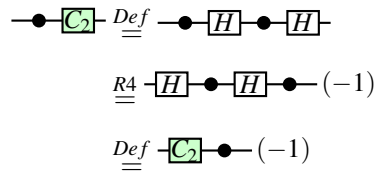

$\oplus$   $\underline{\underline{C}}$   $\stackrel{Def}{=}$   $\boxed{H}$   $\bullet$   $\boxed{H}$   $\boxed{H}$   $\bullet$   $\boxed{H}$  —  
 $\stackrel{R3}{=}$   $\boxed{H}$   $\bullet$   $\bullet$   $\boxed{H}$  —  
 $\stackrel{R2}{=}$   $\boxed{H}$   $\boxed{H}$  —  
 $\stackrel{R3}{=}$  —  
 $\stackrel{Def}{=}$   $\underline{\underline{C}}$  —

## 5.1

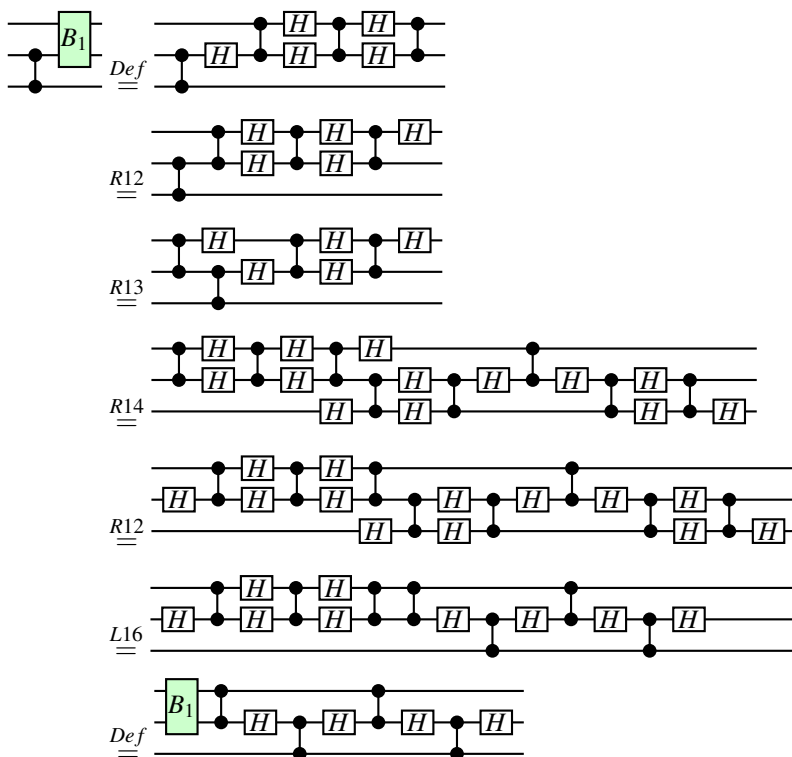

5.2

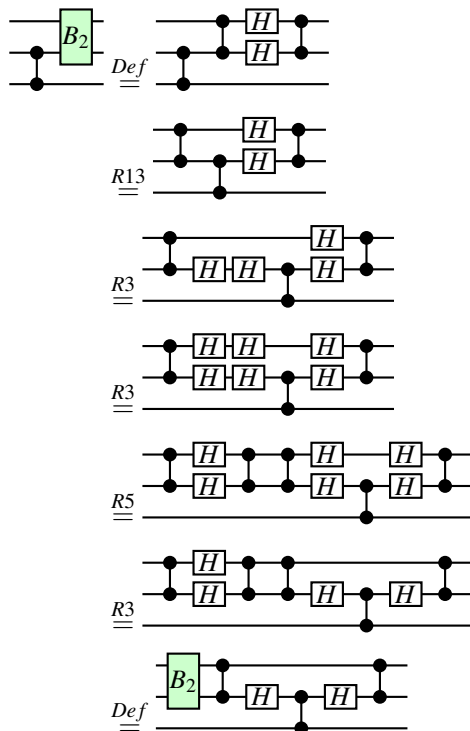

5.3

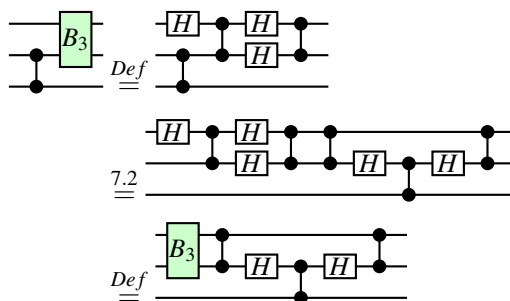

5.4

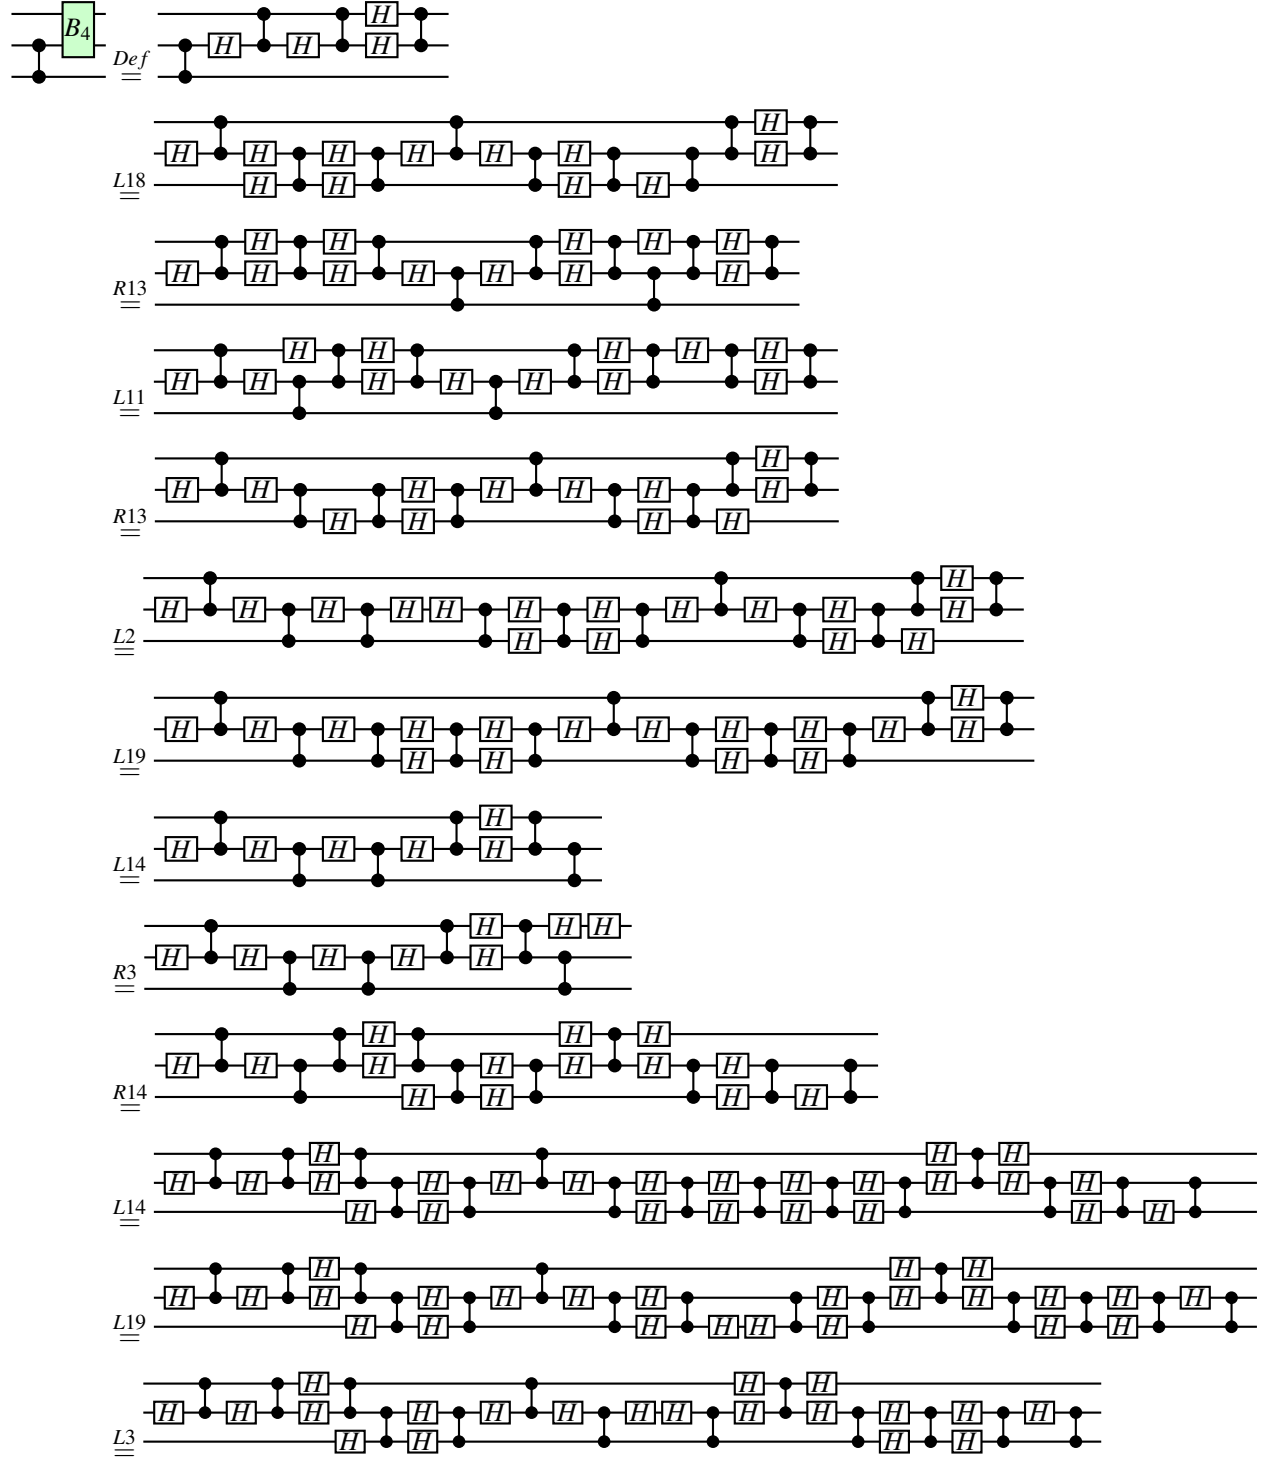

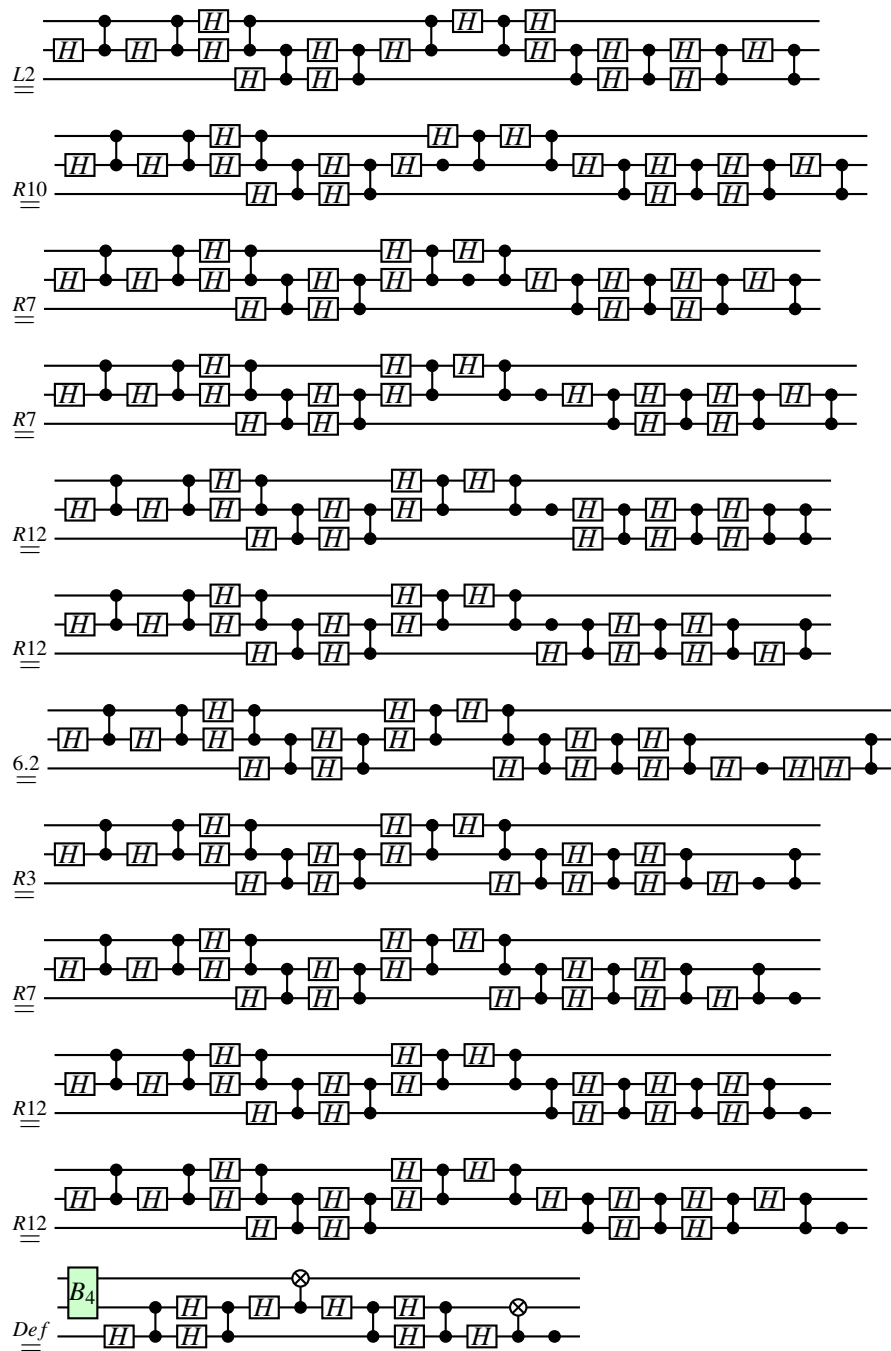

5.5

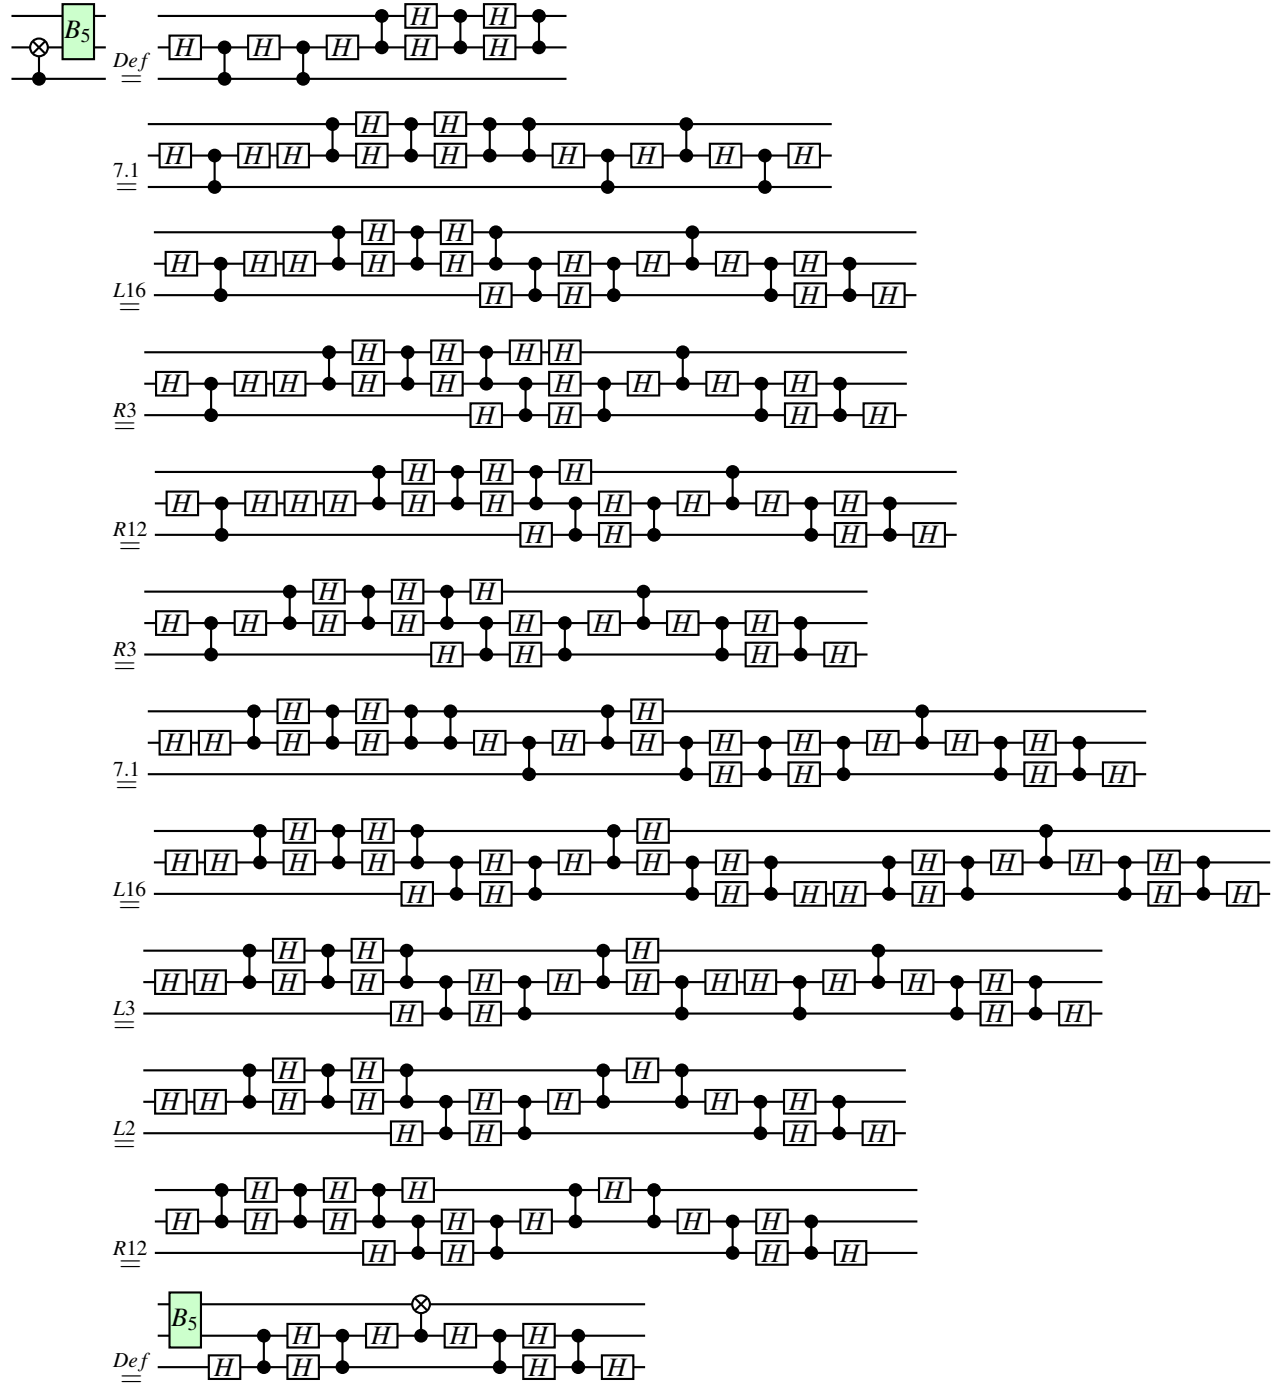

5.6

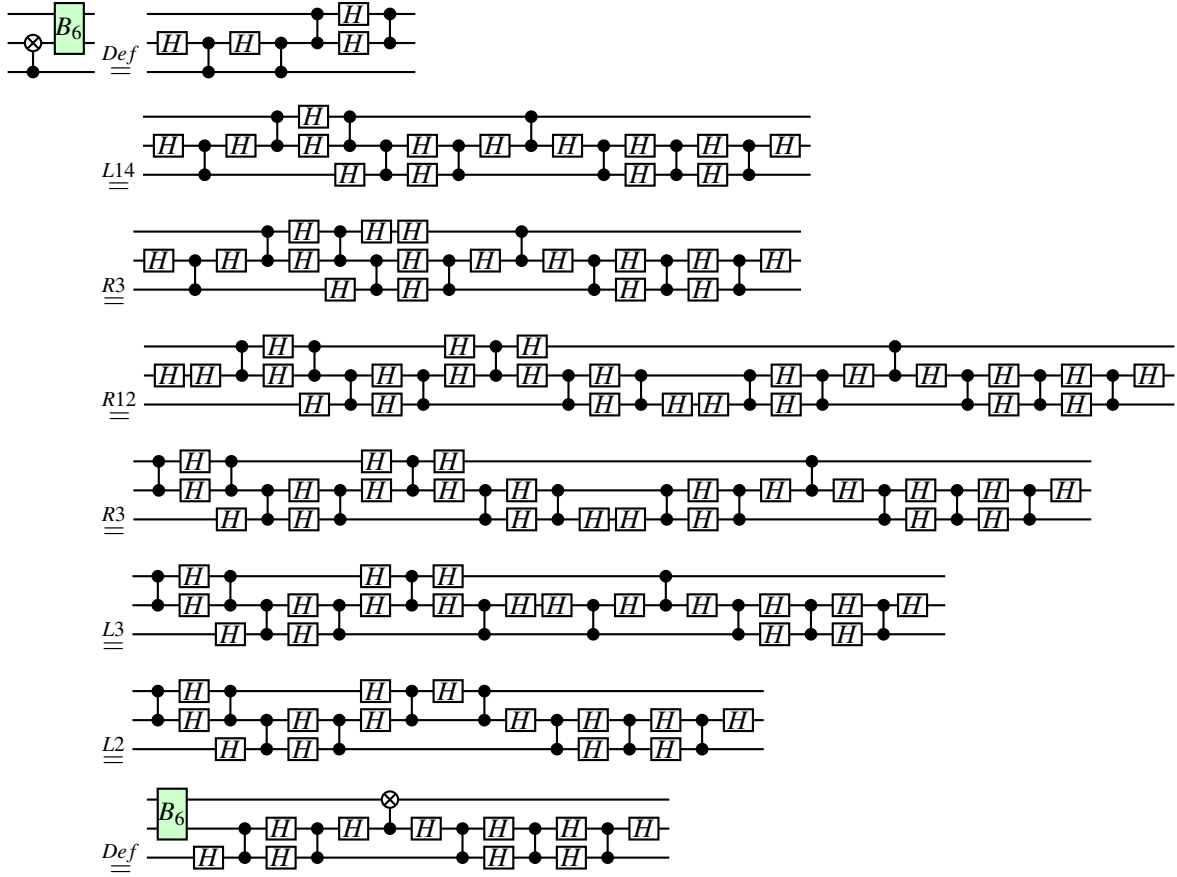

5.7

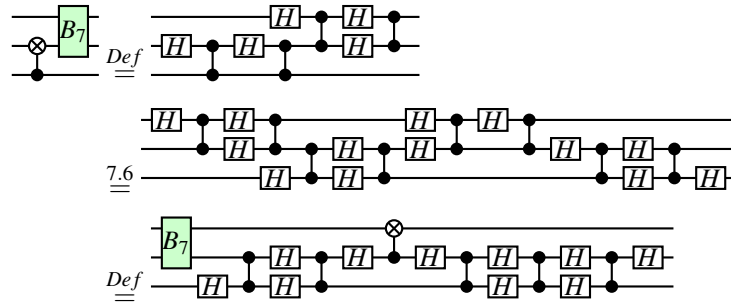

5.8

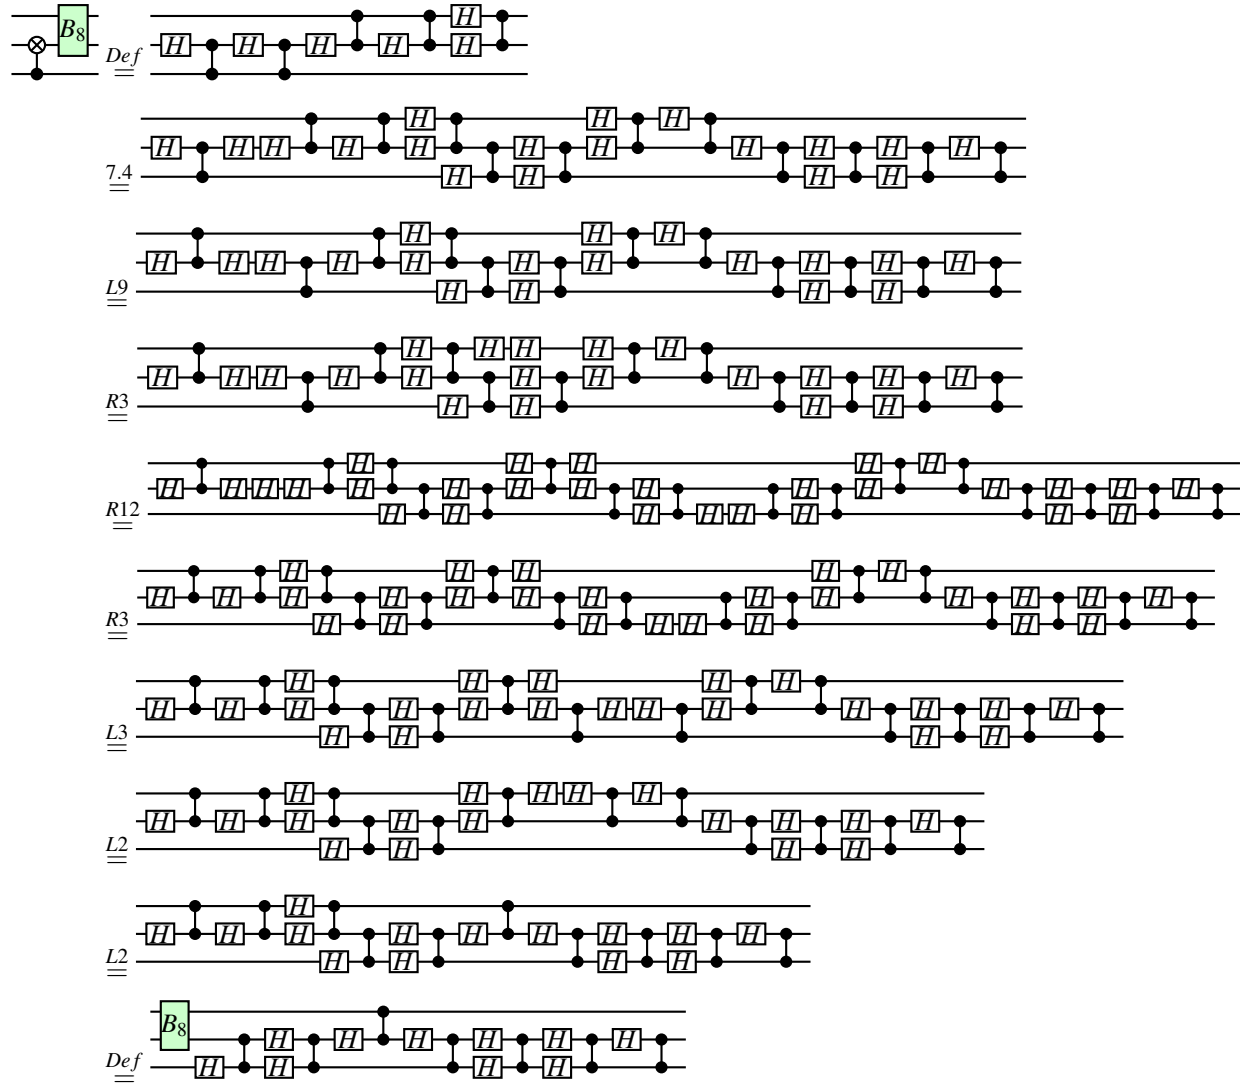

**Figure 6:**

6.1

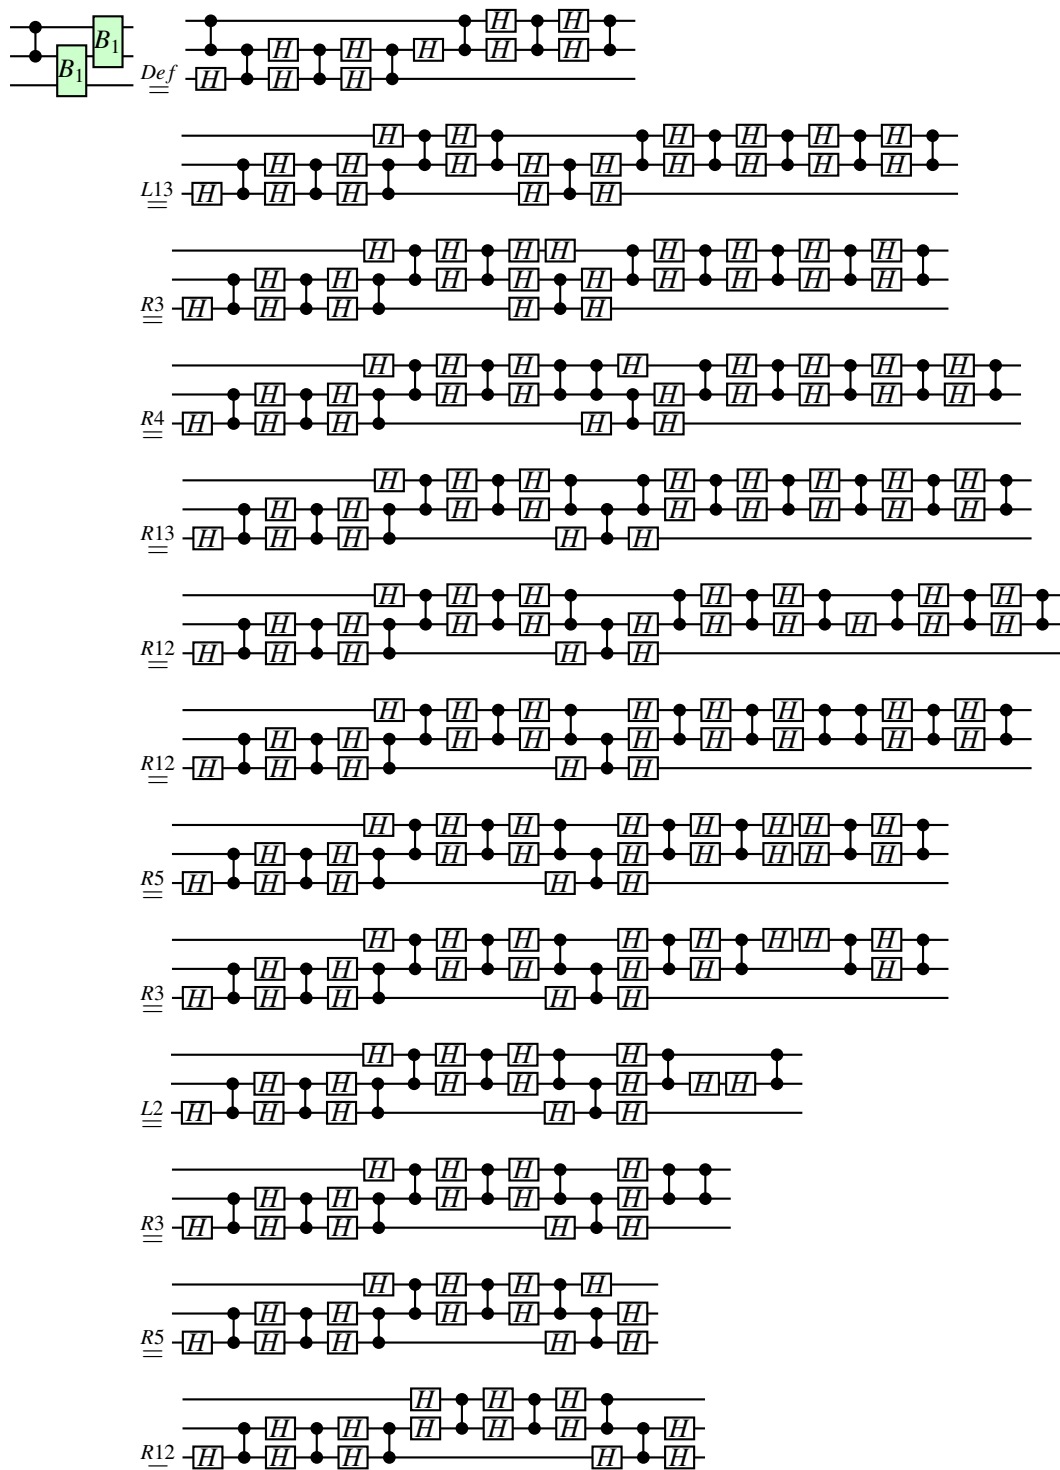

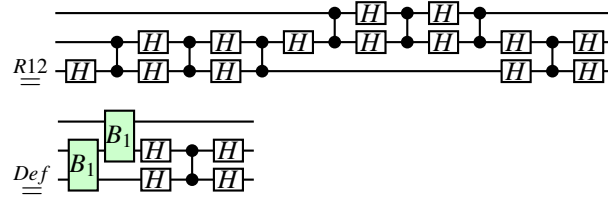

6.2

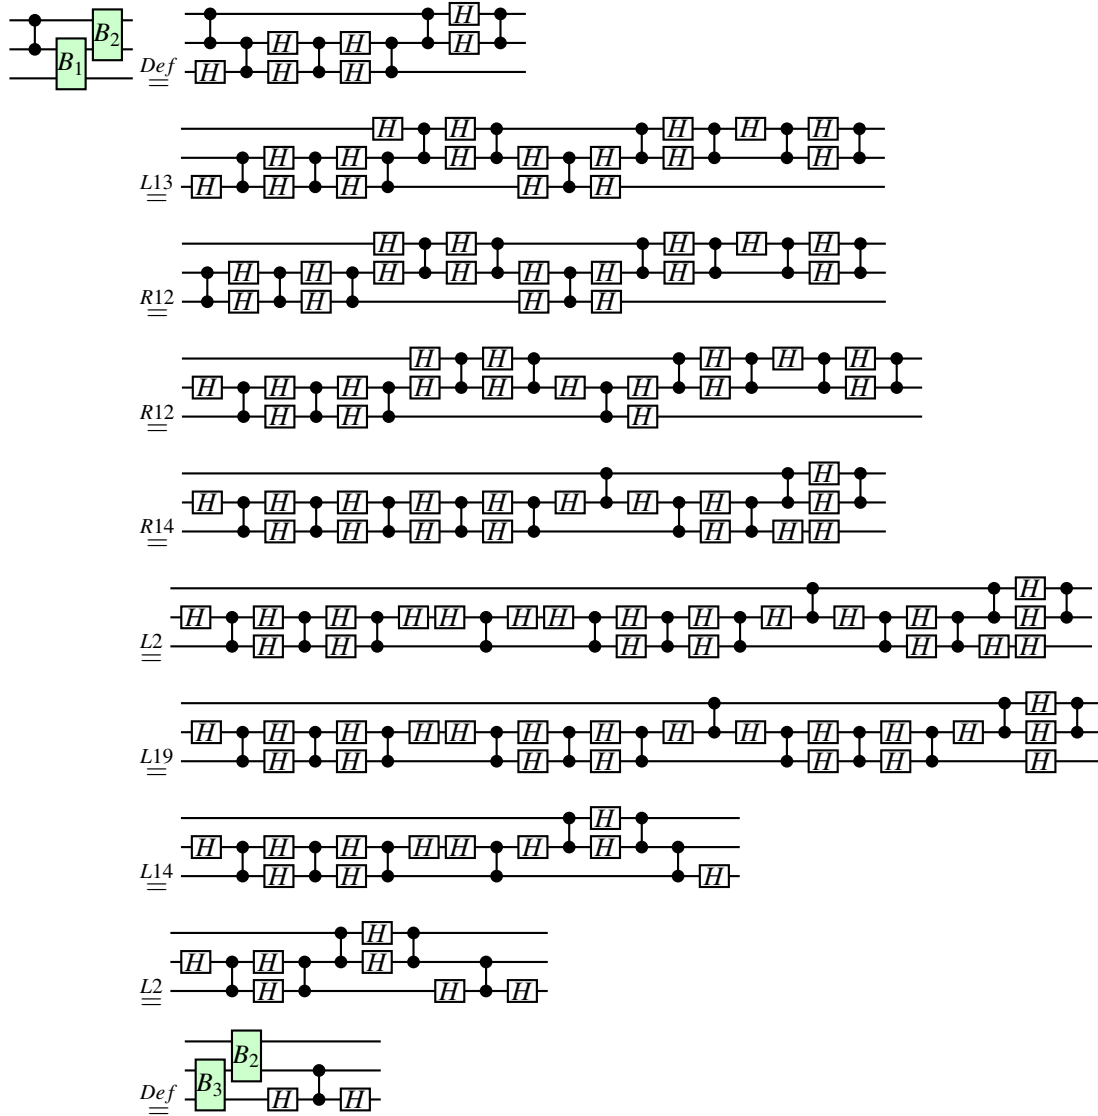

6.3

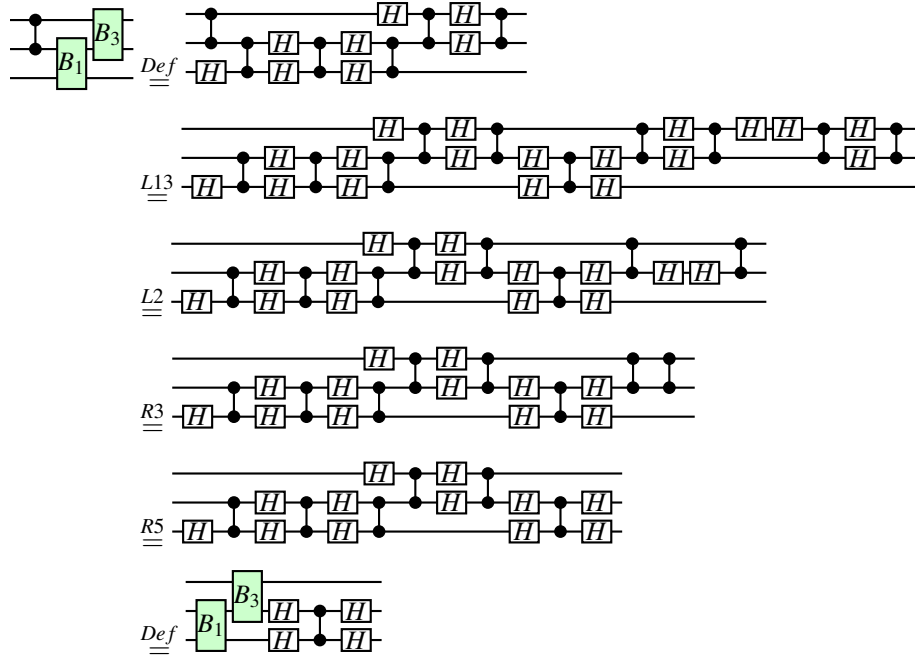

6.4

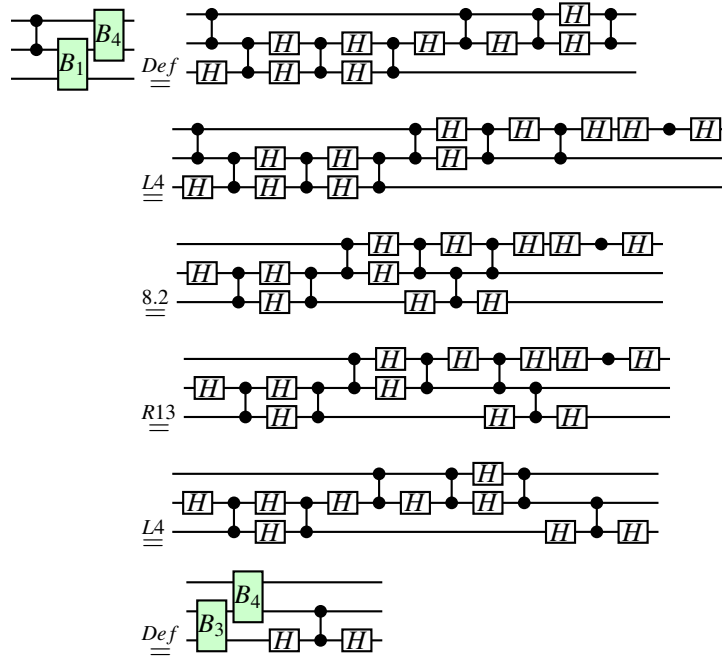

6.5

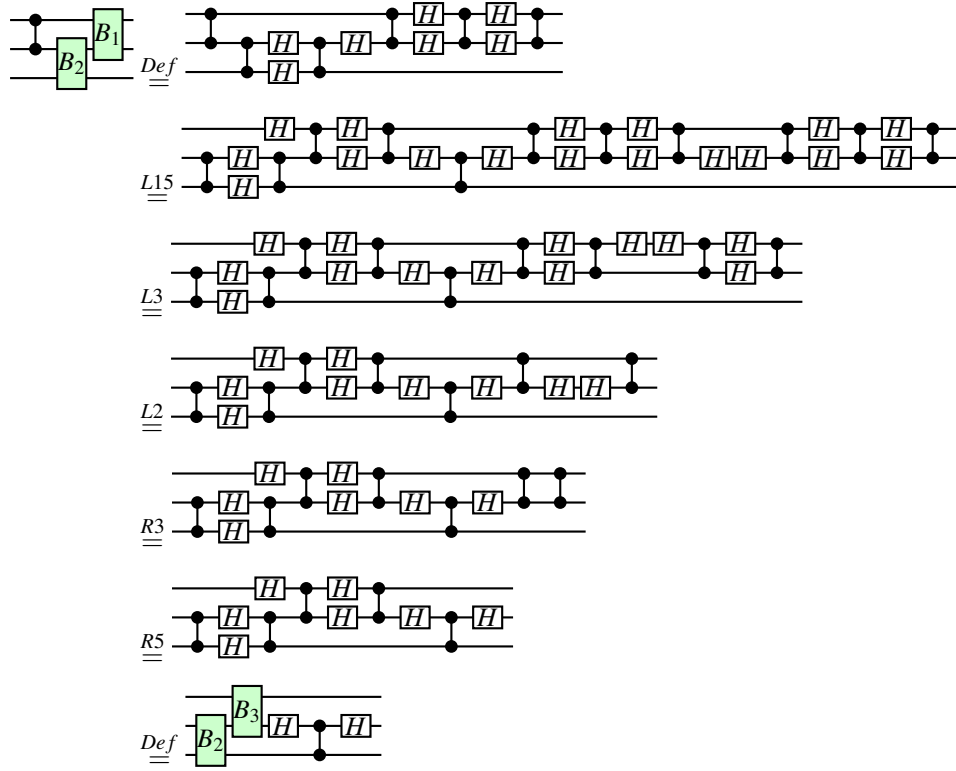

6.6

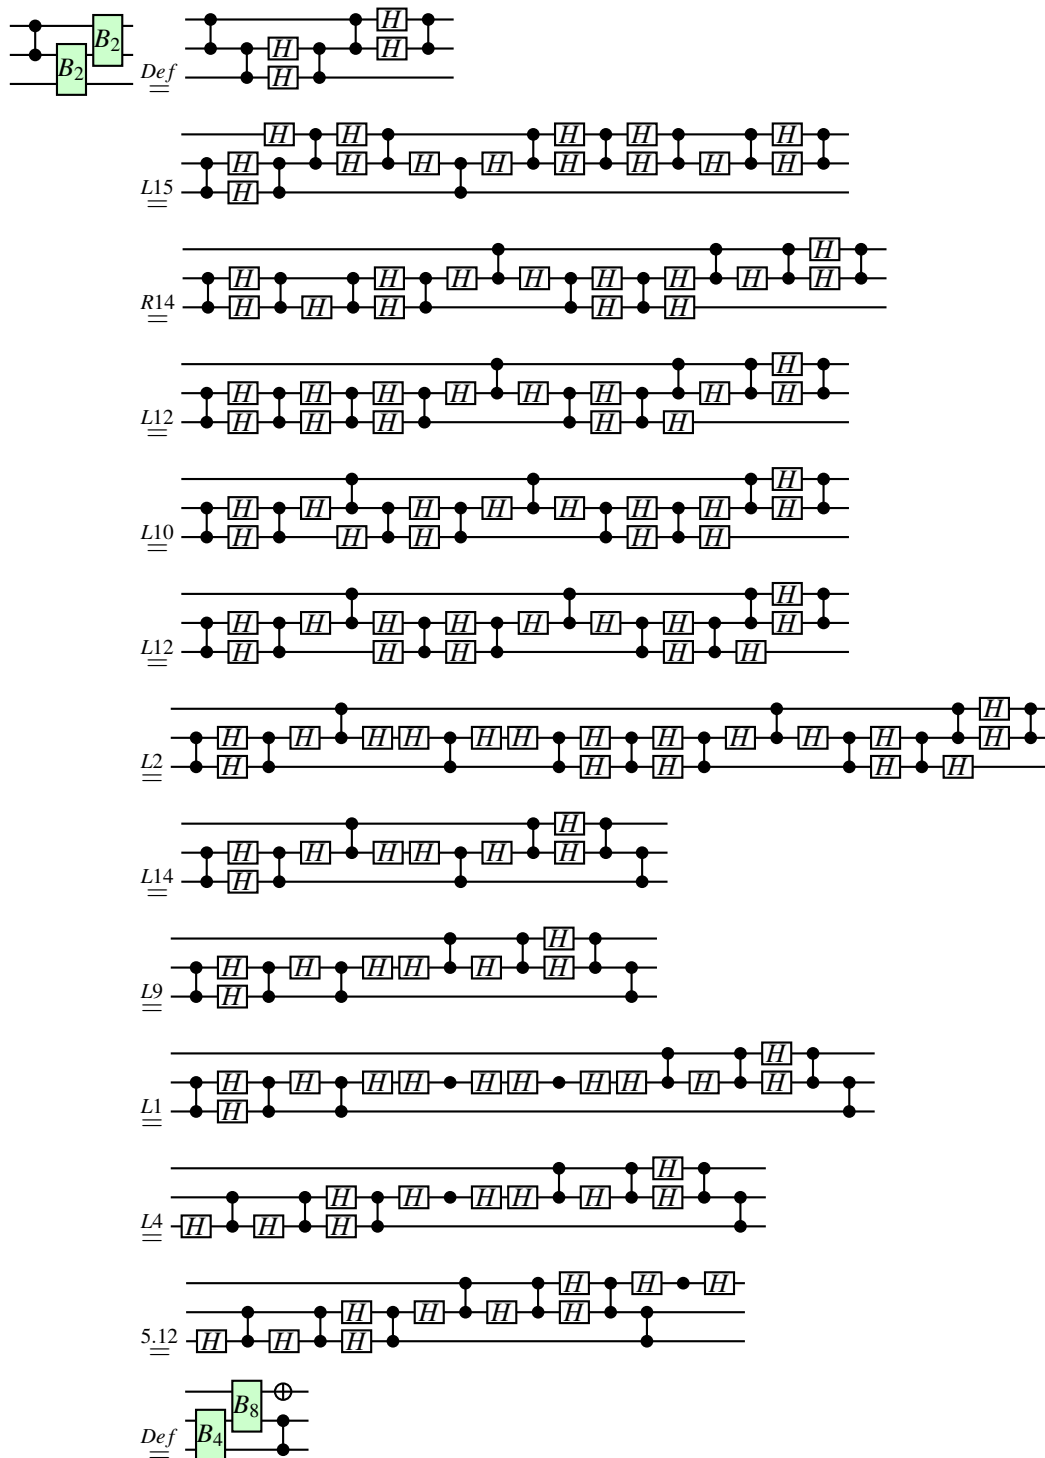

6.7

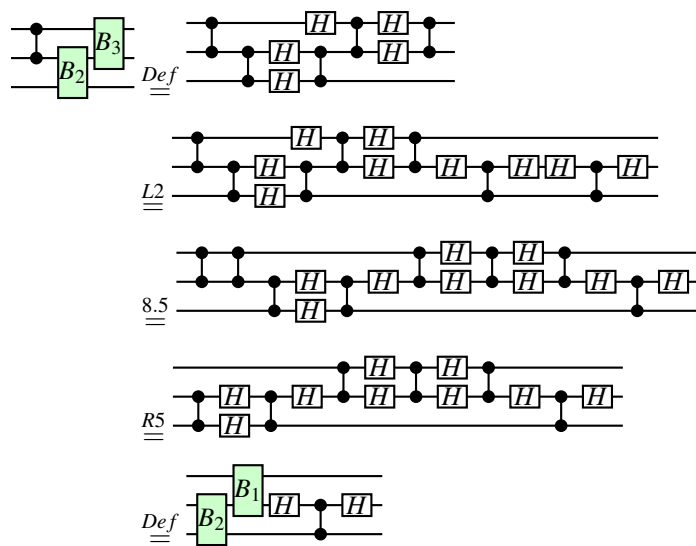

6.8

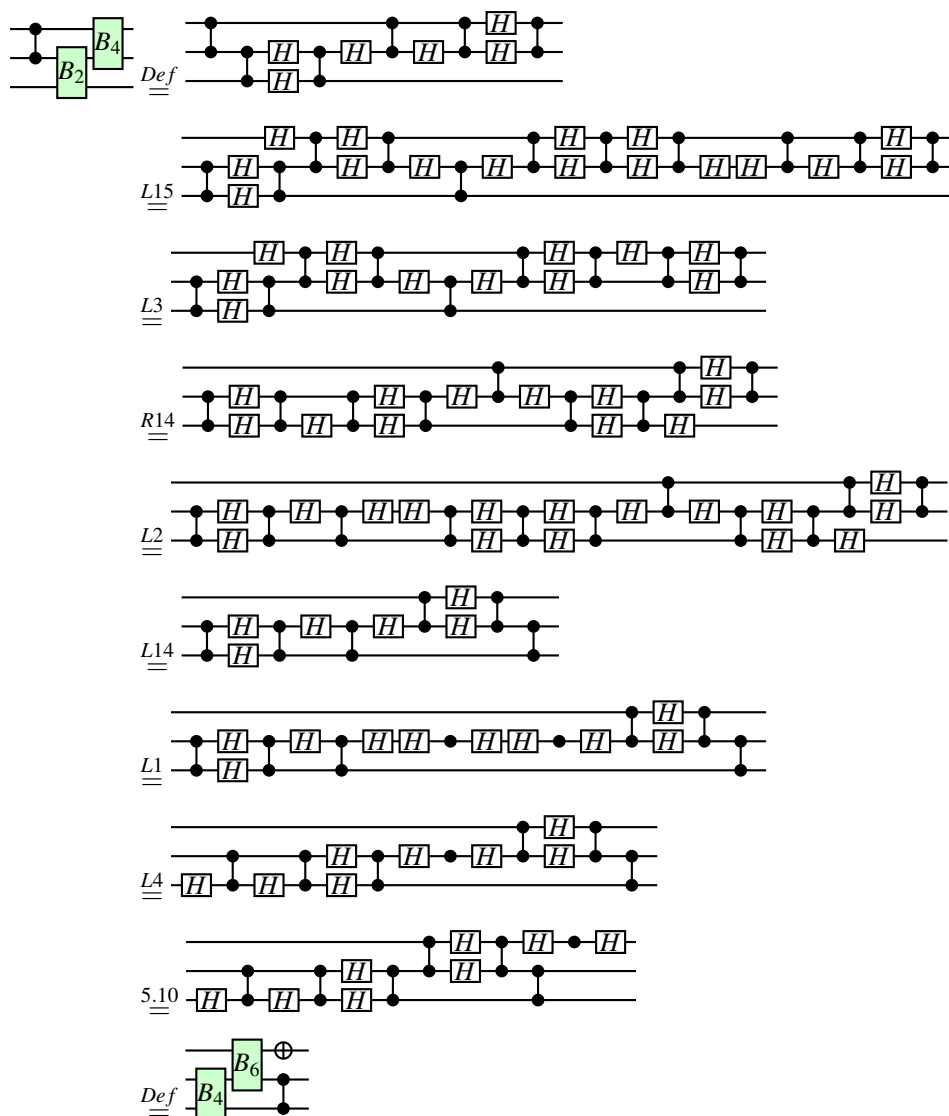

6.9

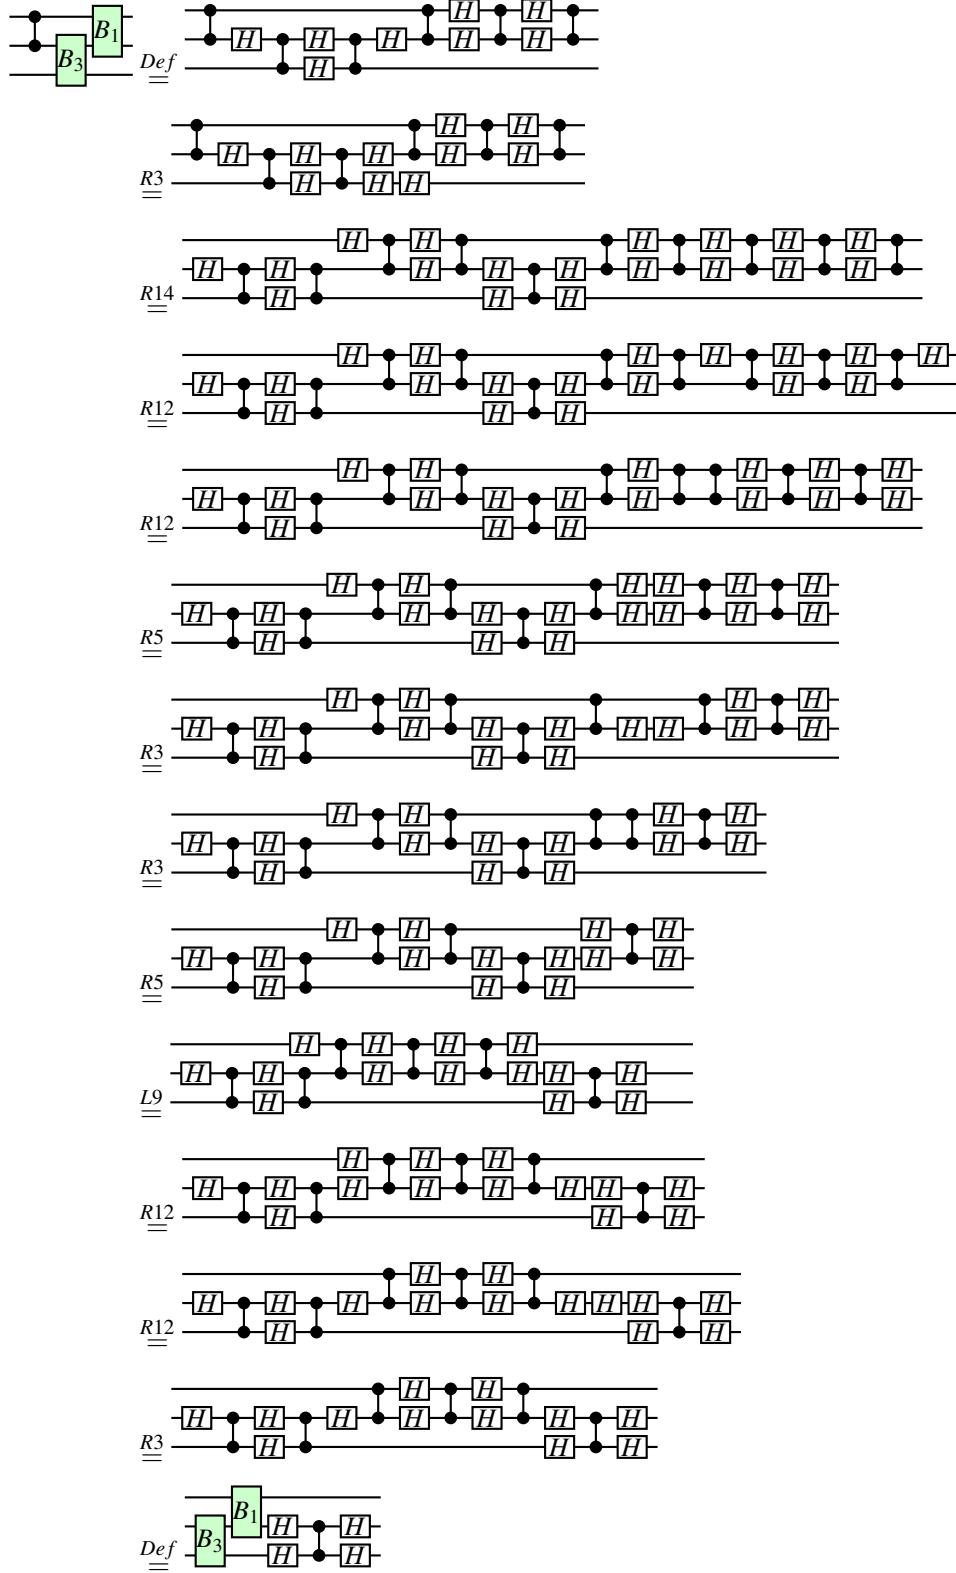

6.10

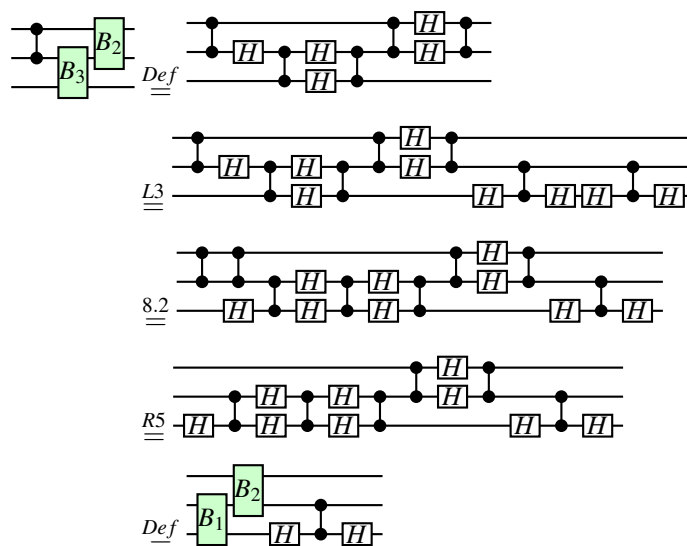

6.11

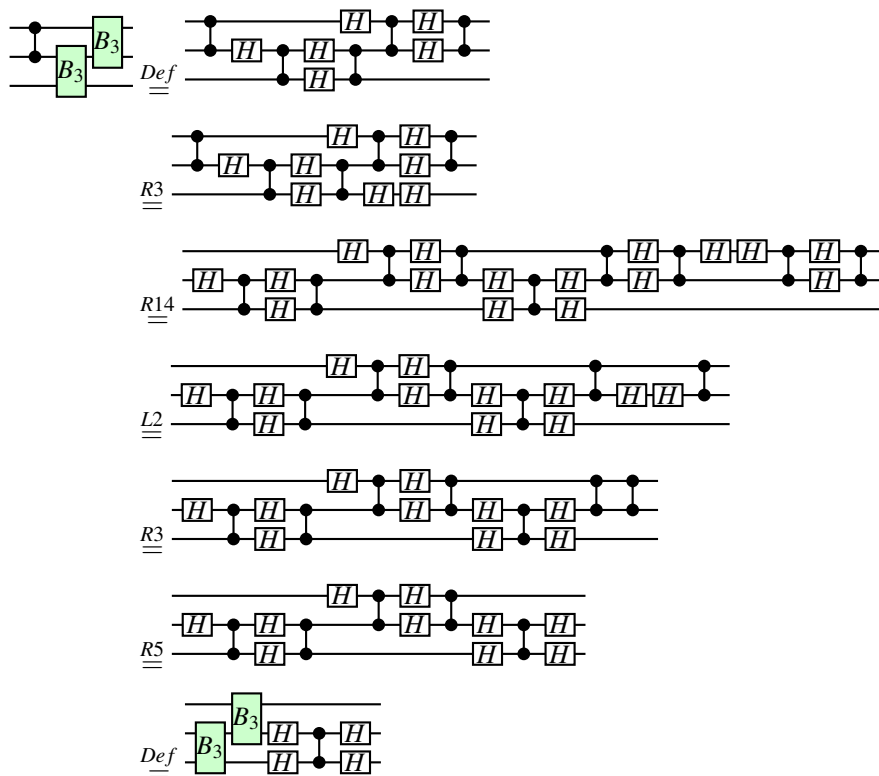

6.12

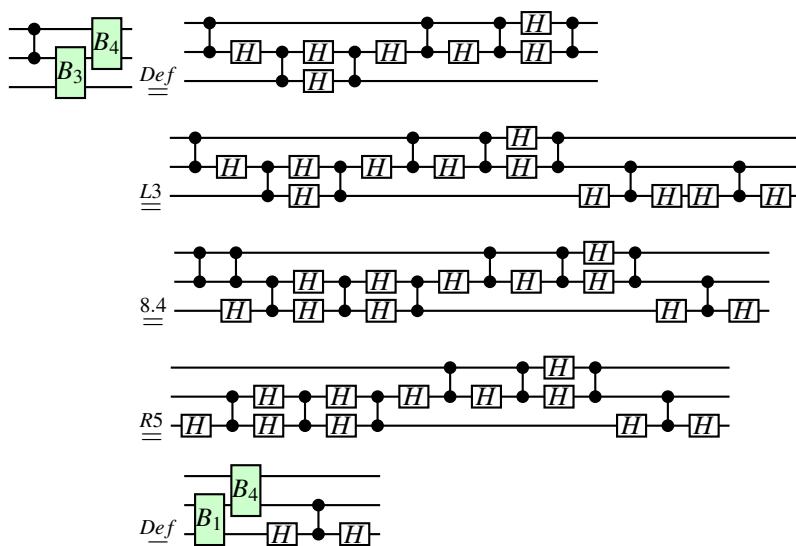

6.13

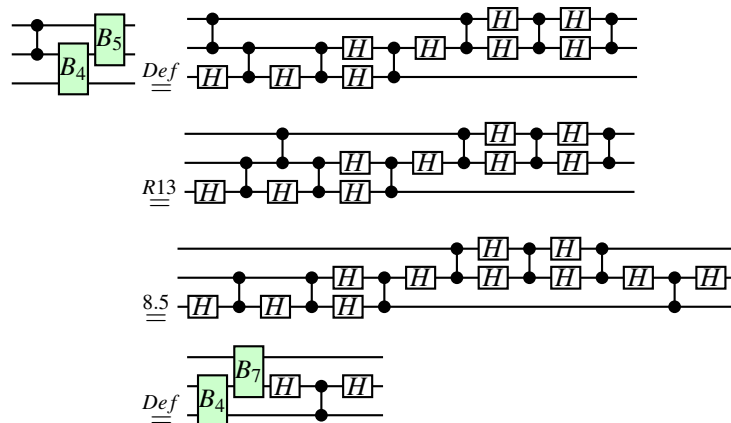

6.14

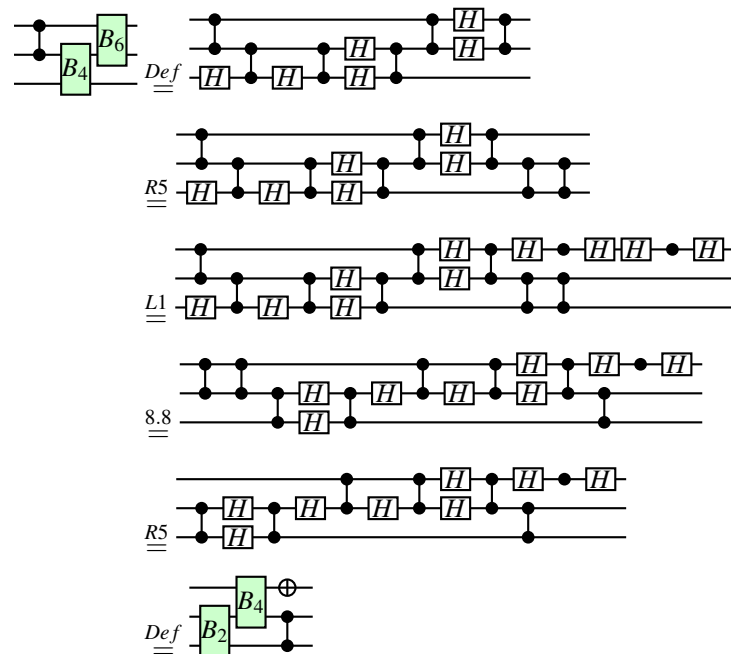

6.15

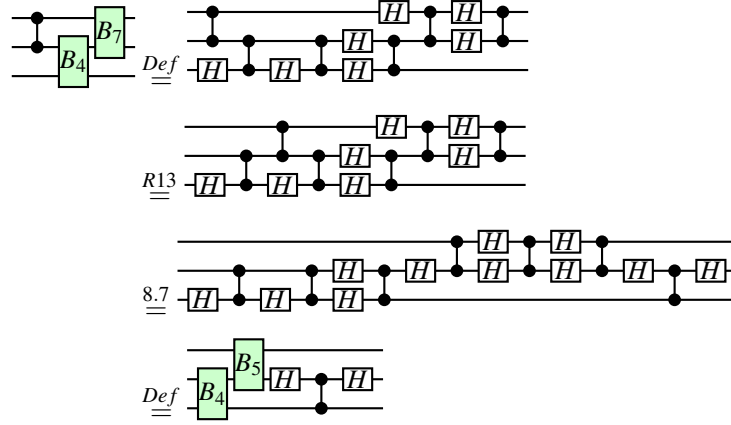

6.16

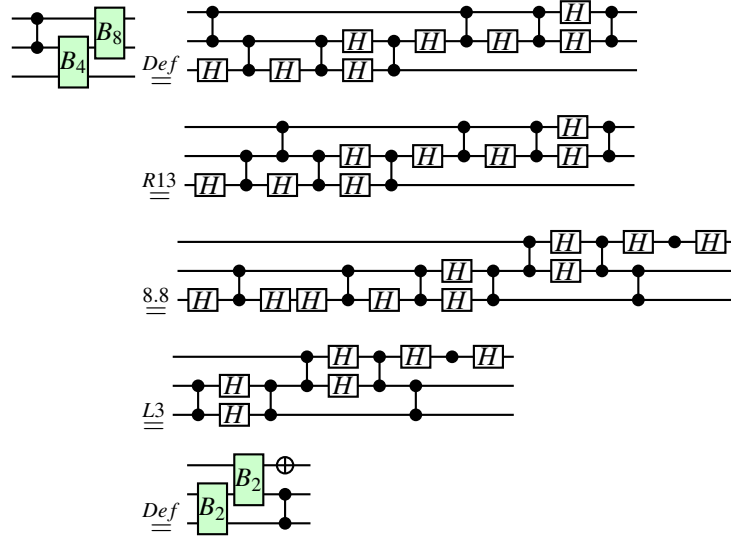**Figure 7:**

The proofs of 7.1–7.16 are the same as those of 6.1–6.16.

**Figure 8:**

8.1

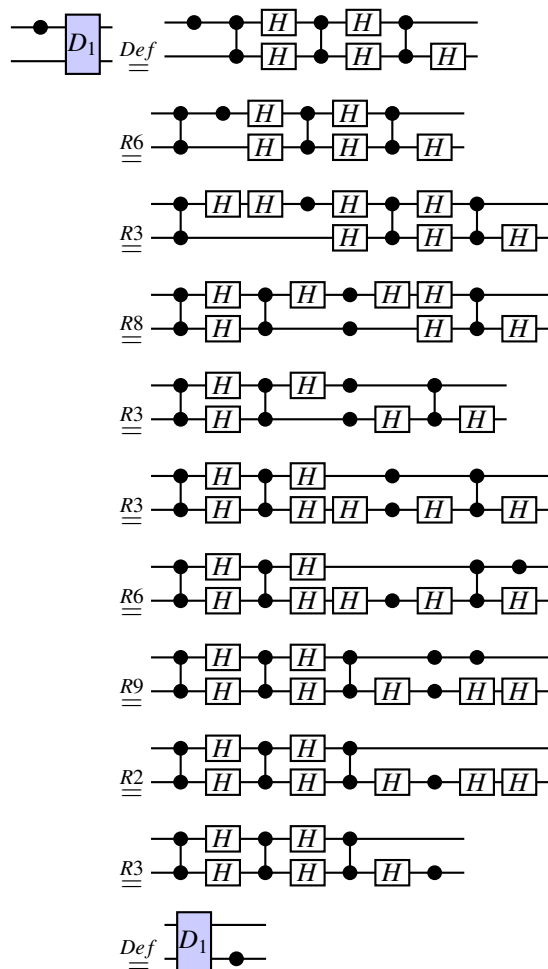

8.2

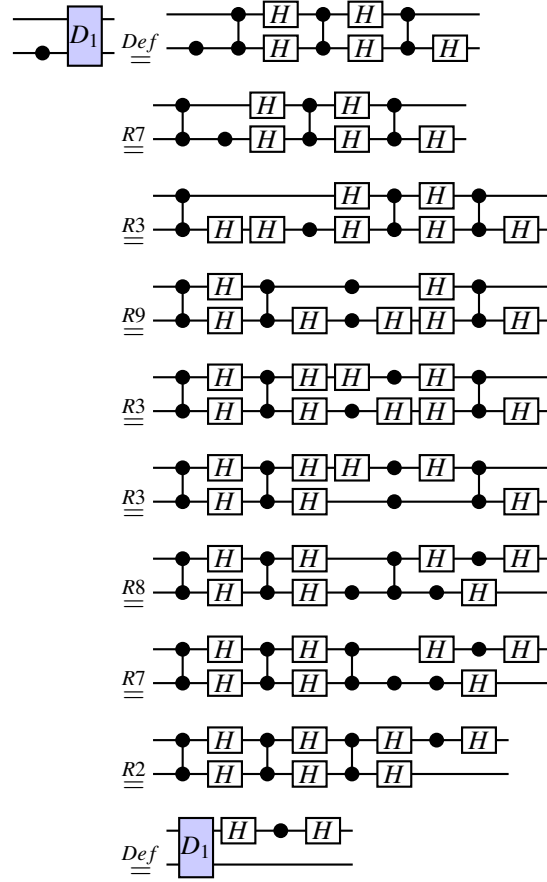

8.3

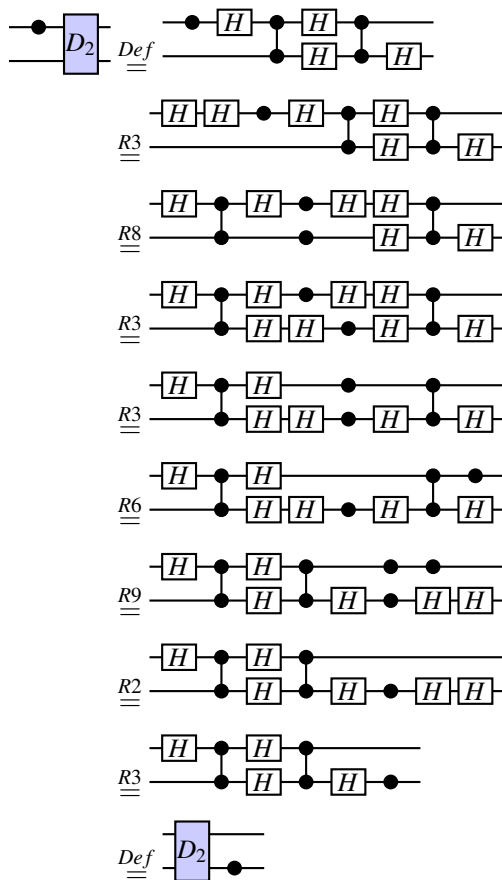

8.4

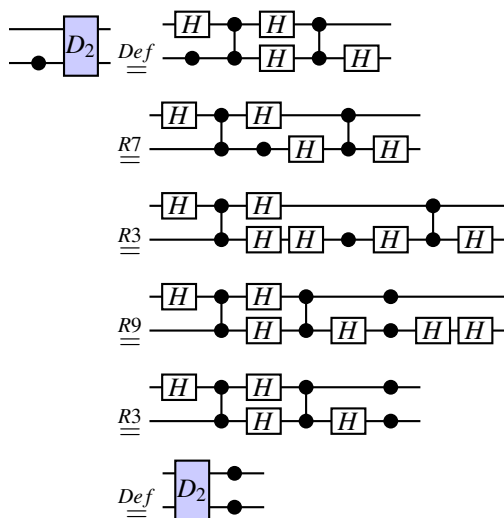

8.5

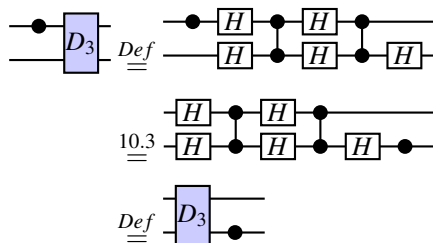

8.6

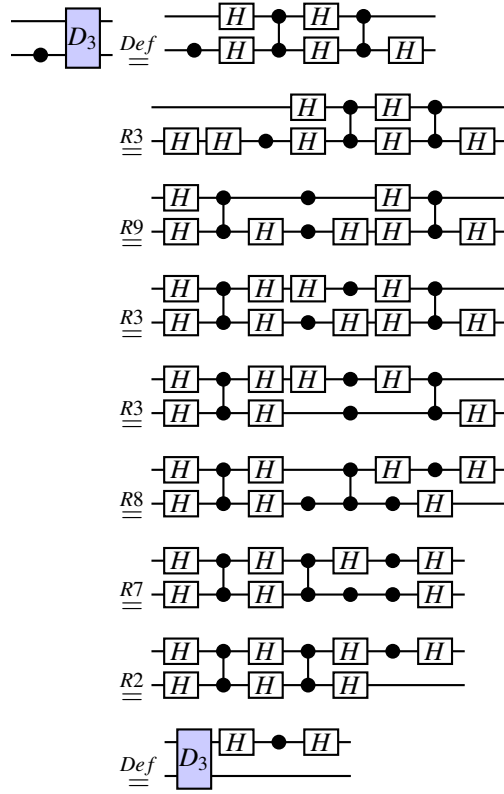

8.7

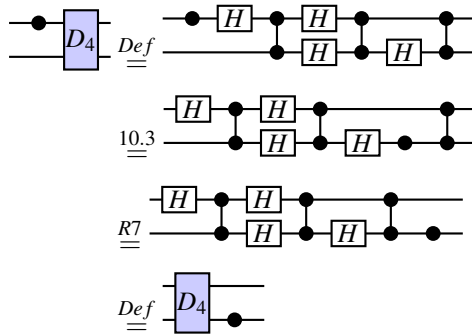

8.8

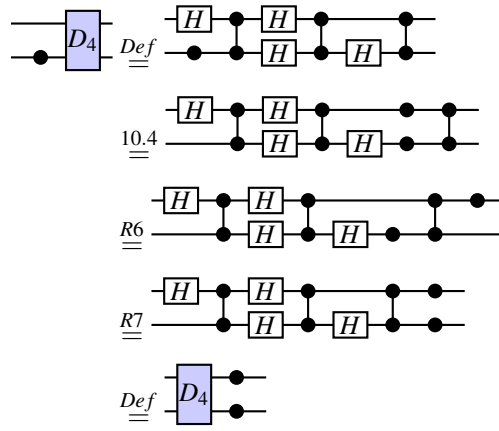

8.9

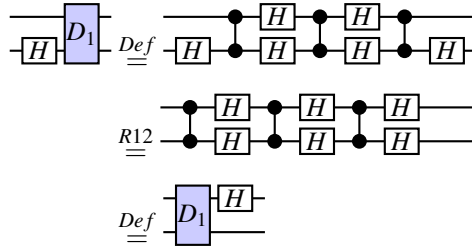

8.10

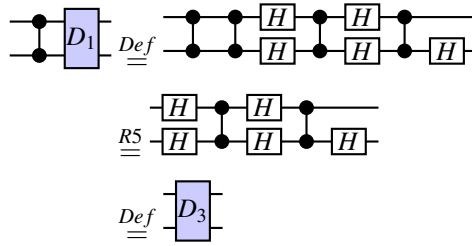

8.11

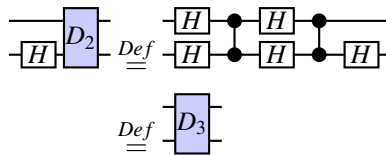

8.12

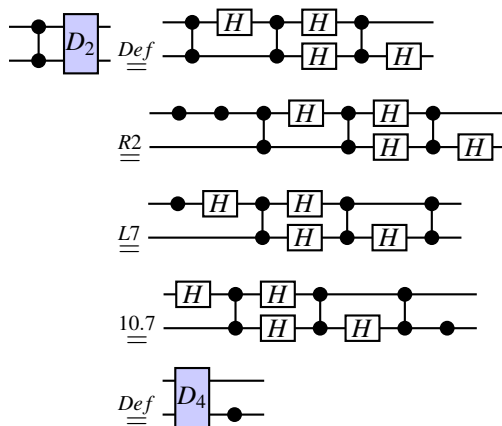

8.13

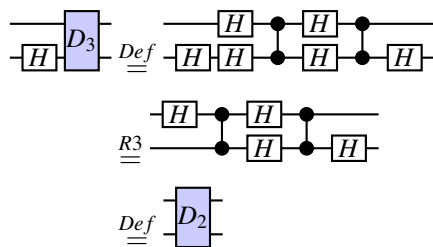

8.14

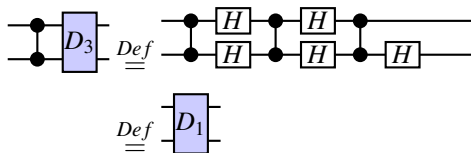

8.15

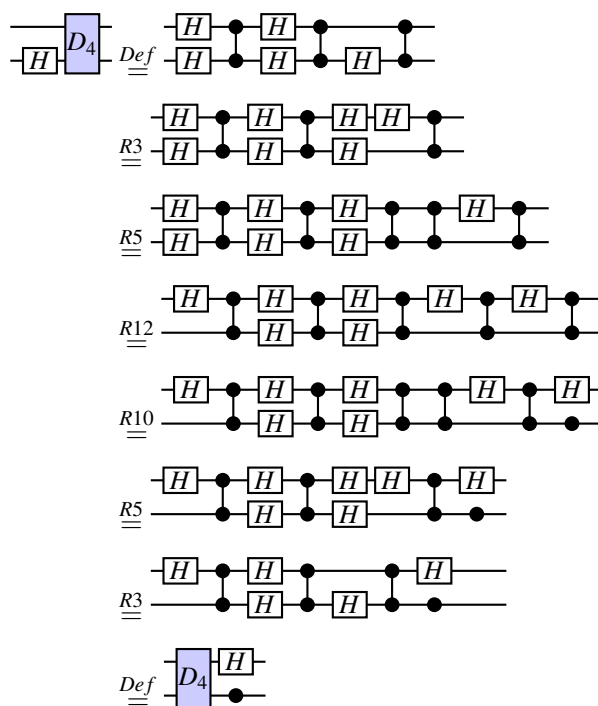

8.16

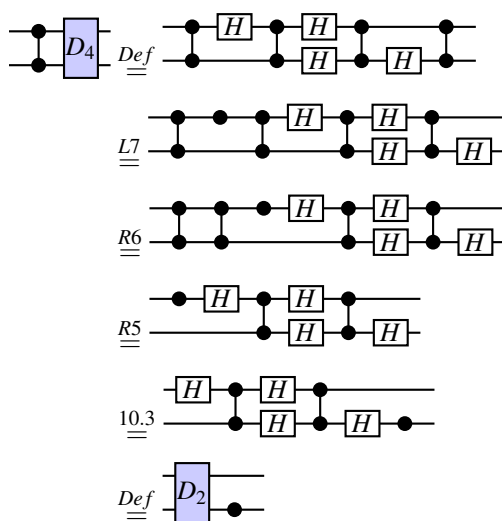

8.17

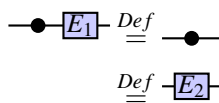

8.18

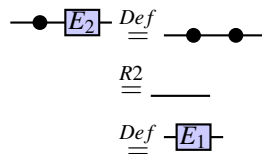

**Figure 9:**

9.1

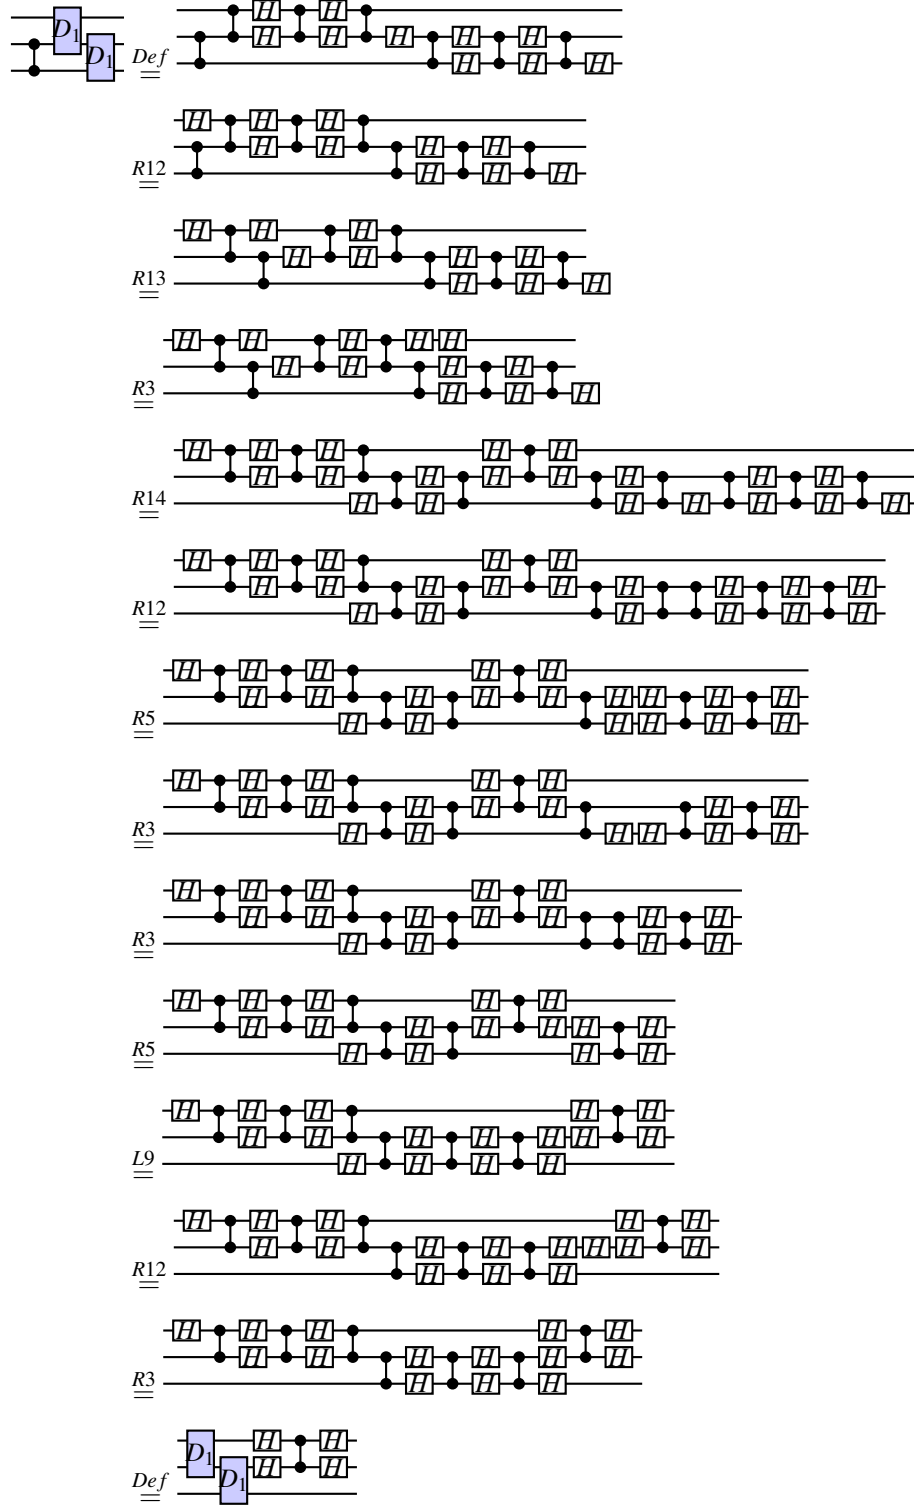

9.2

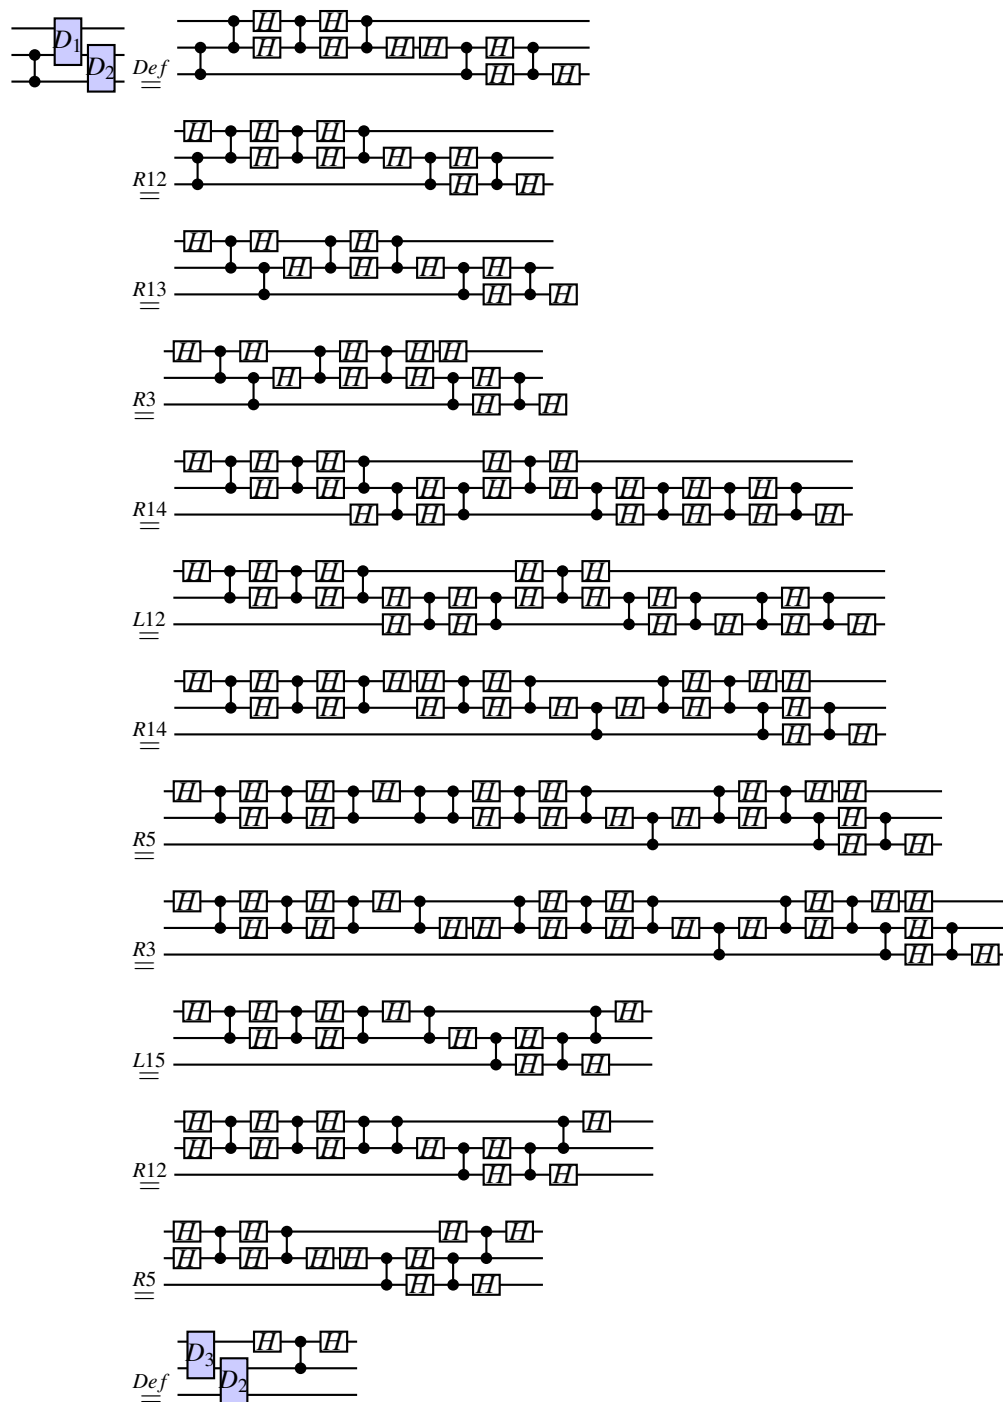

9.3

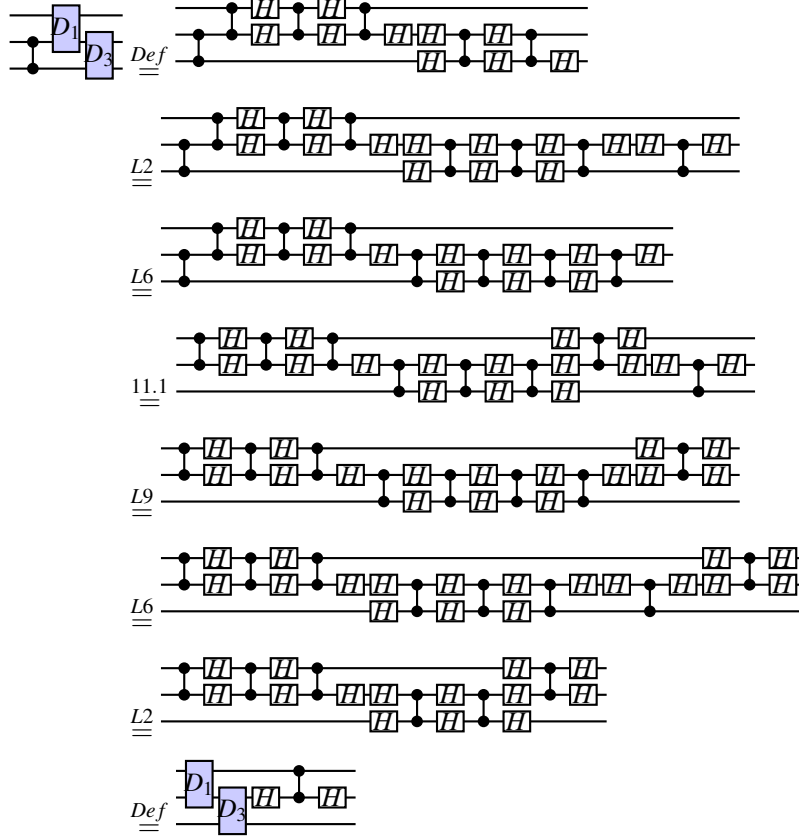

9.4

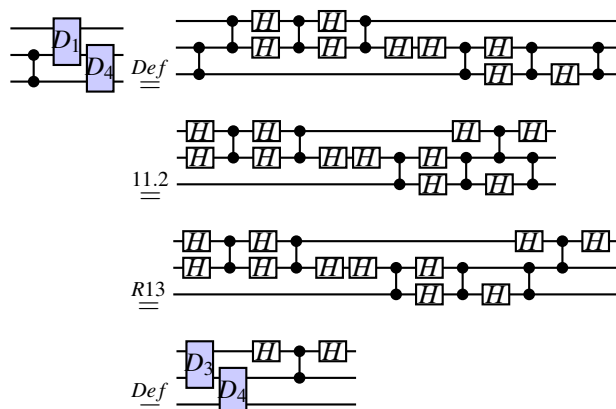

9.5

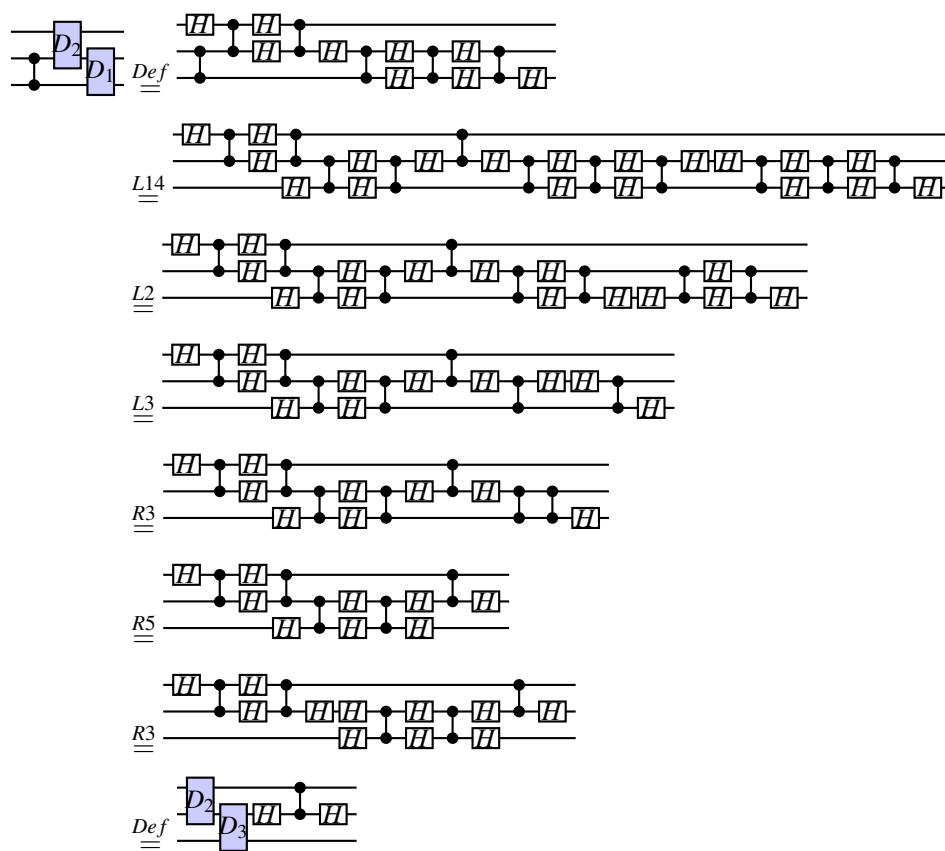

9.6

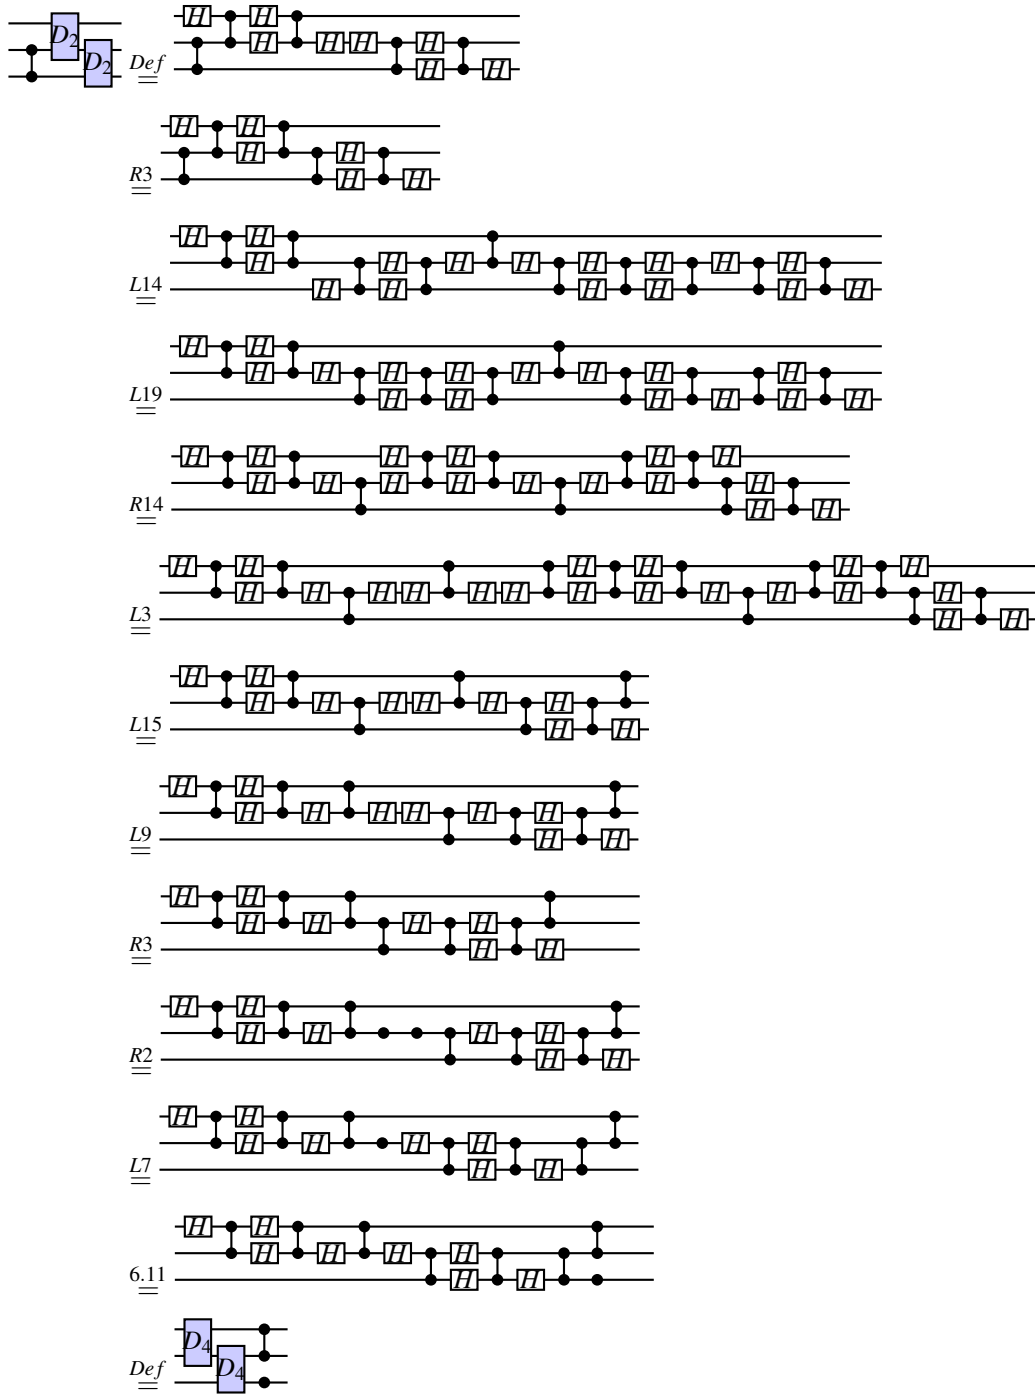

9.7

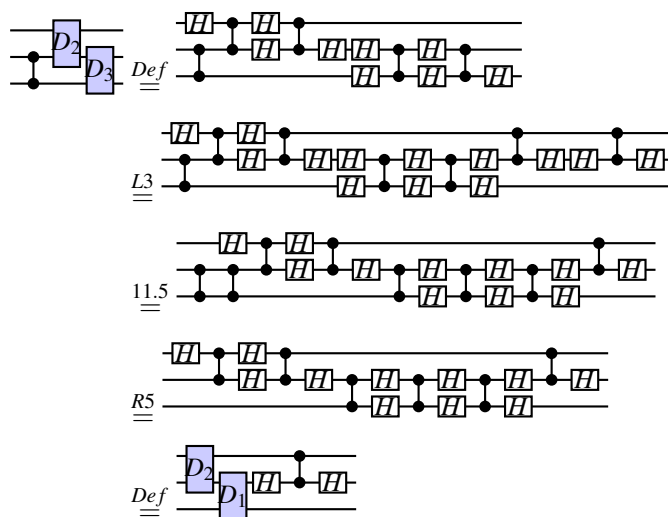

9.8

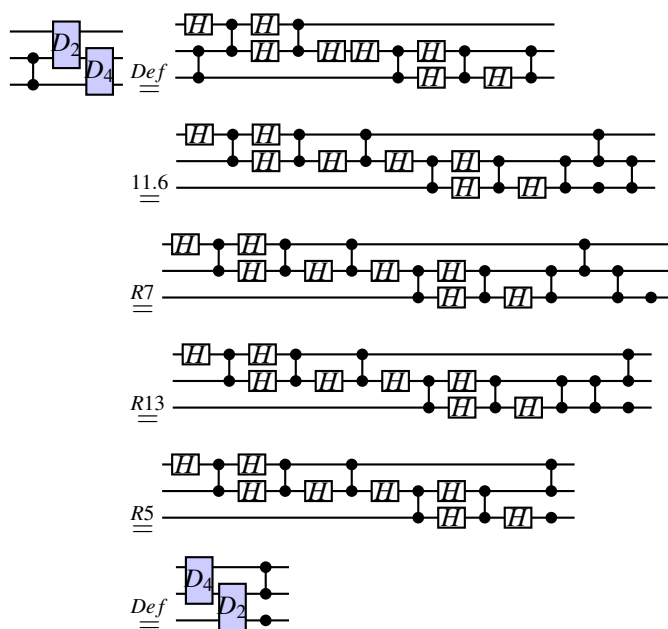

9.9

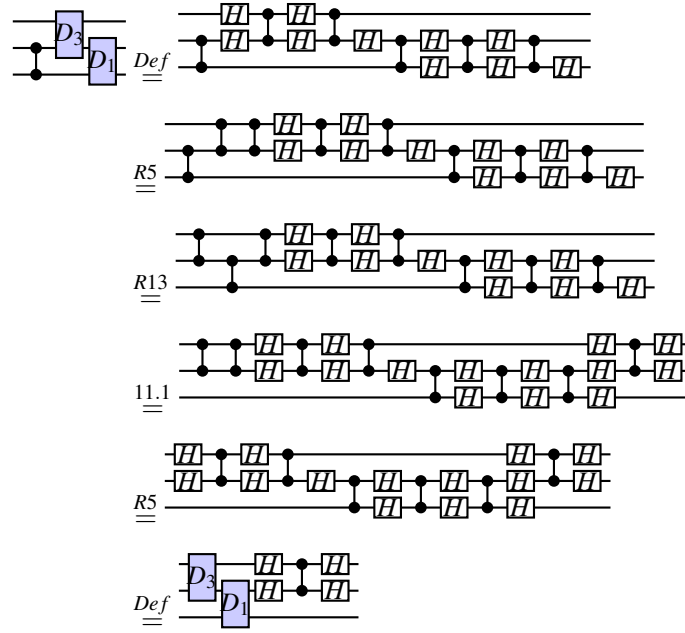

9.10

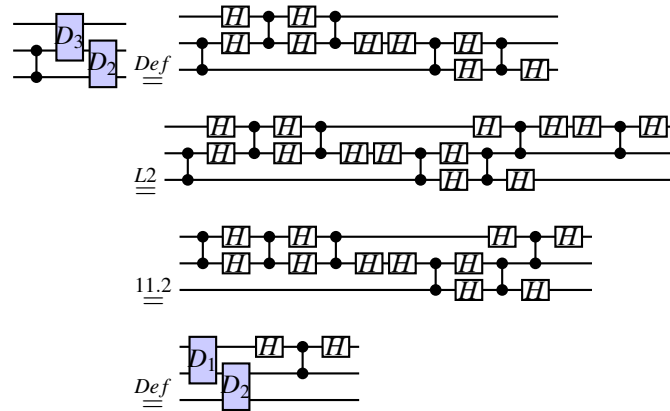

9.11

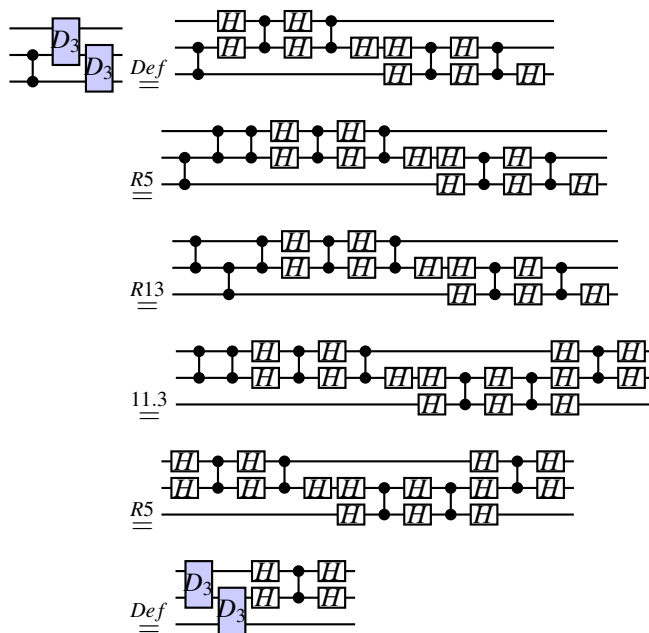

9.12

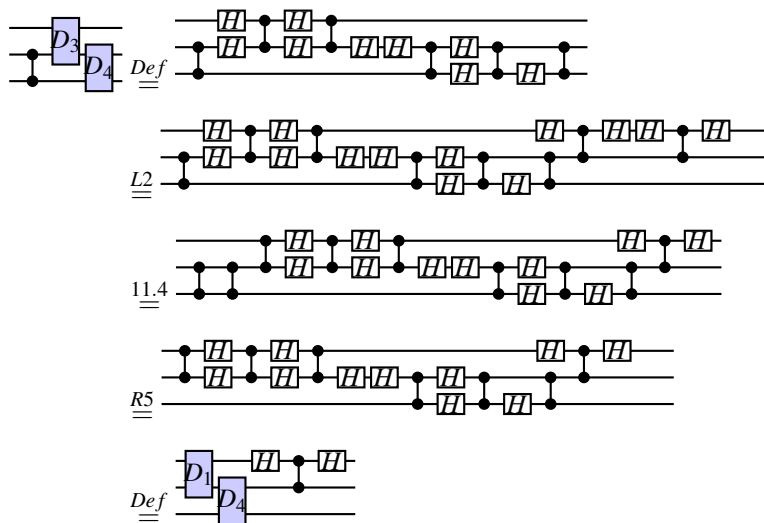

9.13

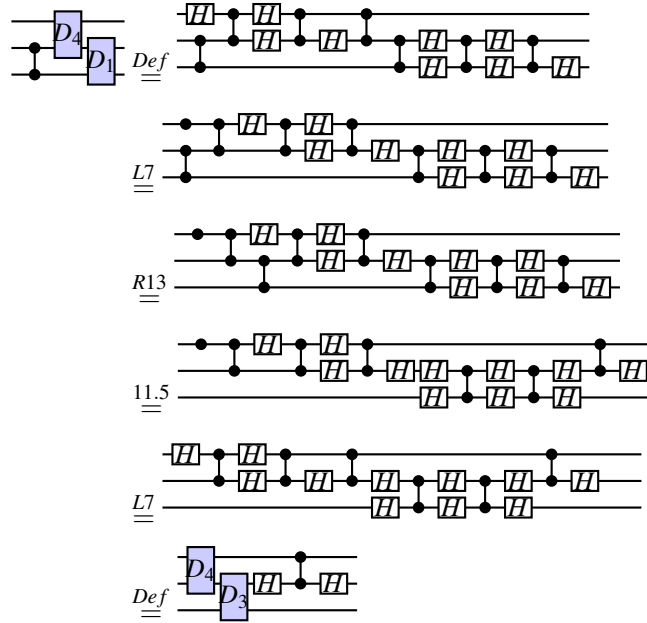

9.14

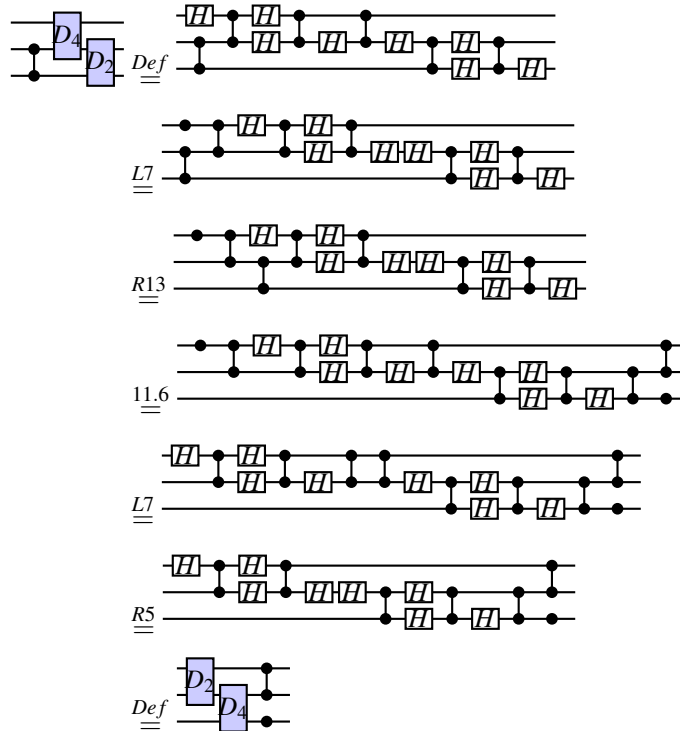

9.15

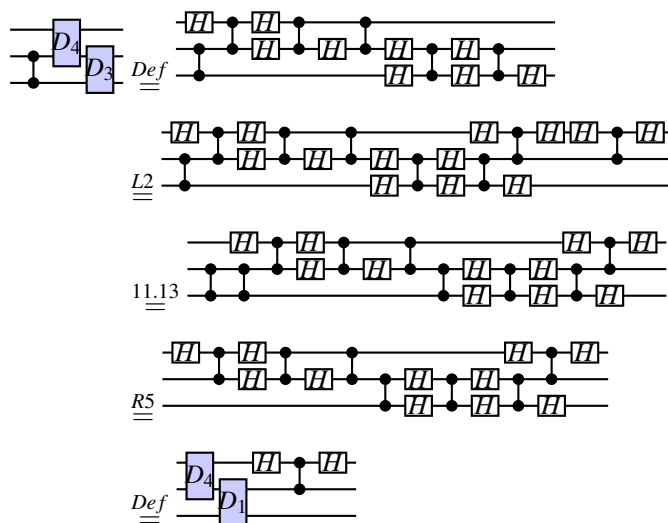

9.16

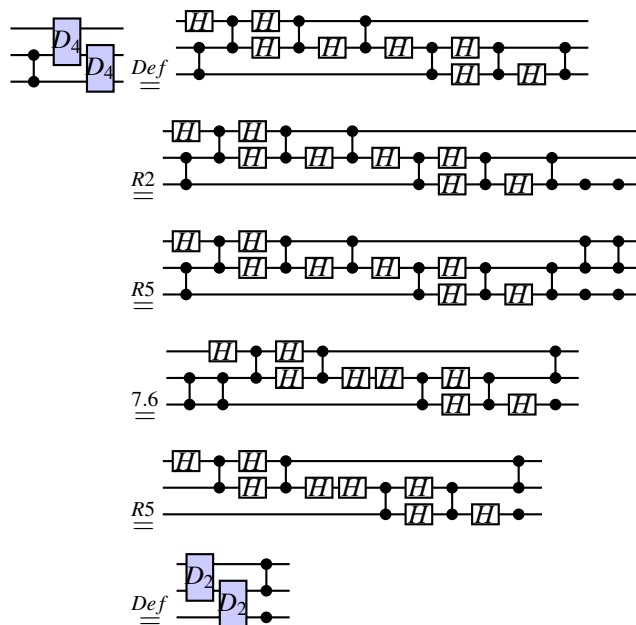**Figure 10:**

10.1

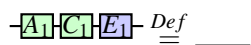

Supplement: Supplementary file 1 [file supplement.pdf]
